# Supplementary material for: Cyclical Long Memory: Decoupling, Modulation, and Modeling
Source: arXiv:2403.07170 source file (2024-07-04)
Supplement: Supplementary file 1 [file Appendix_vol_2.tex]

\section{Definitions of CLM in the ``non-boundary" case} \label{appendix:acvf-spec-clm}
\normalsize

We present the formal definitions for CLM in the time and spectral domain in the non ``boundary" case in Appendix \ref{app:subsec-non-bound-def}, and also state our main result relating the two definitions. In Appendices \ref{app:subsec:time-to-spec} and \ref{app:subsec:spec-to-time}, we prove the result connecting these two definitions of CLM, and in Appendix \ref{subsubsec:admis-phase} we derive the set of admissible phases and mention some special cases. 
% In Section \ref{App:subsec-boundary} we formulate these definitions in the ``boundary" case and provide some conditions connecting these notions. Finally, in Section \ref{app:sec-auxillary} we state and prove some lemmas regarding the second-order behavior of some diverging series and integrals. These Lemmas are used in Section \ref{App:subsec-boundary}. Remark that all definitions and results presented here concern the case of a single singularity in the spectral domain, but analogues for multiple singularities can also be formulated. 

\subsection{Time and spectral domain definitions} \label{app:subsec-non-bound-def}

We first recall two definitions related to slowly varying functions. A slowly varying function $L:[0, \infty) \to (0,\infty)$ at infinity is called \textit{quasi-monotone} (see, e.g., Chapter 2.7 in \cite{bingham_goldie_teugels_1987}) if the following two conditions hold: $(i)$ it is of bounded variation on any compact interval of $[0,\infty)$ and $(ii)$ for some $\delta > 0$,
\[
\int_0^x u^\delta |d L(u)| = O(x^\delta L(x)), \quad \text{as } x \to \infty.
\]
A measurable function $f$ \textit{belongs to the Zygmund class} if, for every $\alpha > 0$, $x^\alpha f(x)$ is ultimately increasing and $x^{-\alpha} f(x)$ is ultimately decreasing, i.e., there exists some $M \in \RR_+$ such that $x^{\alpha} f(x)$ is increasing in $[M,\infty)$ (resp. $x^{-\alpha} f(x)$ is decreasing in $[M,\infty)$). The Zygmund class coincides with that of the normalized slowly varying functions, see, e.g., Chapter 1.5.3 of \cite{bingham_goldie_teugels_1987}. We use the following convention for the sign function of a constant $c \in \RR$:
\[
\text{sign}(c) = \begin{cases}
    1 & c \ge 0, \\
    -1 & c < 0.
\end{cases}
\]

\begin{defn}(Time domain) \label{defn:clm-time}
    A second-order stationary time series $\{X_n\}_{n \in \ZZ}$ is said to exhibit CLM if its autocovariance function satisfies 
    \begin{align} \label{eq:def-eq-acvf} 
       \gamma_X(h) = L_{1,\gamma}(h) \cos(\lambda_0 h) h^{2d-1} + \xi L_{2,\gamma}(h) \sin(\lambda_0 h) h^{2d-1} , \quad h \ge 0, 
    \end{align}
    where $ \lambda_0 \in (0,\pi), \xi = \pm 1$, and $d \in (0,1/2)$ are constants, and $L_{1,\gamma}, L_{2,\gamma} : [0,\infty) \to (0,\infty)$ are slowly varying functions with $L_{1,\gamma}(x) \sim c_{1,\gamma} \in (0,\infty)$ and $\xi L_{2,\gamma}(x) \sim c_{2,\gamma} \in \RR$ as $x \to \infty$ (clearly $\xi =  \operatorname{sign}(c_{2,\gamma})$) and
    \begin{equation} \label{eq:def-c1g-c2g}
    c_{1,\gamma} \in \RR_+ \; \text{and} \; c_{2,\gamma} = 0, \quad \text{or} \quad 
    \frac{c_{1,\gamma}}{c_{2,\gamma}} \in (-\tan(\pi d), \tan(\pi d))\footnote{check that we want it closed here}.
     \end{equation}
\end{defn}

The next remark provides an alternative  useful formulation for CLM in the time domain. 

\begin{remark} \label{rmk-clm-defn-time-equiv}
   The relation \eqref{eq:def-eq-acvf} can be recast as
    \begin{equation} \label{def-time-2}
    \gamma_X(h) = c_\gamma \cos(\lambda_0 h + \phi)  h^{2d-1} + R(h),
    \end{equation}
    where
    \begin{equation} \label{eq:rig-c1g-c2g-c-psi}
    \begin{split}
         c_\gamma &\doteq \sqrt{(c_{1,\gamma})^2 + (c_{2,\gamma})^2}, \\
         \phi &\doteq \arcsin\left(  \frac{-  c_{2,\gamma}}{\sqrt{(c_{1,\gamma})^2 + (c_{2,\gamma})^2}}\right) \in \left( -\left(\frac{1}{2} - d \right) \pi, \left(\frac{1}{2} - d\right) \pi \right)\footnote{check open or closed},
    \end{split}
    \end{equation}
    and 
    \begin{equation}
    \begin{split}
     R(h) &\doteq (L_{1,\gamma}(h) - c_{1,\gamma}) \cos(\lambda_0 h ) h^{2d-1} + ( \xi L_{2,\gamma}(h) - c_{2,\gamma}) \sin(\lambda_0 h ) h^{2d-1} \\
     &= \cos(\lambda_0 h ) o(h^{2d-1}) + \sin(\lambda_0 h ) o(h^{2d-1}).
    \end{split}
    \end{equation}
\end{remark}

\begin{defn}(Spectral domain) \label{defn:clm-spec}
    A second-order stationary time series $\{X_n\}_{n \in \ZZ}$ is said to exhibit CLM if its spectral density satisfies
\begin{equation} \label{eq:spec-rigorous-defn}
    f_X(\lambda) = \begin{cases}
        L_f^- \left(\frac{1}{\lambda_0 - \lambda}\right)  (\lambda_0 - \lambda)^{-2d}, & 0 < \lambda < \lambda_0, \vspace{3mm}\\
        L_f^+ \left(\frac{1}{\lambda - \lambda_0}\right)  (\lambda - \lambda_0)^{-2d}, & \lambda_0 < \lambda < \pi,
    \end{cases}
\end{equation}
where $\lambda_0 \in (0,\pi), d \in \left( 0, \frac{1}{2} \right)$, and $L_f^-: \left(\frac{1}{\lambda_0},\infty\right) \to (0,\infty)$ and $L_f^+: \left(\frac{1}{\pi - \lambda_0},\infty\right) \to (0,\infty)$  are two slowly varying functions at $\infty$ such that $L_f^+(x) \sim c_f^+$ and $L_f^-(x)  \sim c_f^-$ as $x \to + \infty$, where $c_f^\pm \in (0,\infty)$.
\end{defn}

Definitions \ref{defn:clm-time} and \ref{defn:clm-spec} are, in general, not equivalent. We are aware of only two works relating these two definitions (or variations of them). First, in Proposition 2 of \cite{viadenopp95}, an argument is provided for passing from the spectral to the time domain definition for extended fractional ARMA processes with seasonal effects\footnote{Vladas: check the reference, they exhibit CLM} in the ``non-boundary" case. However, even for this specific class of processes, the reader is referred to a different, but similar proof, and so the arguemnts are not complete. Second, Lemma 1 of Chapter 2 in \cite{phdArt98} considers an argument for passing from the spectral to the time domain definition in the ``boundary" case (see Appendix \ref{App:subsec-boundary} below). While the proof strategy is valid (and, in fact, similar to the one used in Appendix \ref{App:subsec-boundary}), it ignores second-order asymptotic expansions (see Appendix \ref{app:sec-auxillary}), thus rendering the stated result imprecise. We are not aware of any results obtaining a spectral domain representation from the time domain. 

We now formulate a result that establishes the connection between these two definitions in the ``non-boundary" case $\phi \in \left( -\left( \frac{1}{2} -d \right) \pi, \left( \frac{1}{2} -d \right) \pi \right)$. We emphasize that special treatment is required for the ``boundary" case $\phi = \pm \left( \frac{1}{2} -d \right) \pi$; see Appendix \ref{App:subsec-boundary}.

\begin{proposition} \label{prop:equiv-defn} \text{}

\begin{enumerate}[(i)]
    \item Suppose that $L_{1,\gamma}, L_{2,\gamma}$ are slowly varying, \PZ{quasi-monotonic functions} at $+ \infty$.
    % Suppose, moreover, that either $c_{1,\gamma} \in \RR_+$ and $c_{2,\gamma} = 0$ or that $\frac{c_{1,\gamma}}{c_{2,\gamma}} \in( - \tan(\pi d),\tan(\pi d)) $. 
    Then, Definition \ref{defn:clm-time} implies Definition \ref{defn:clm-spec} with 
    % $L_f^+(x)  \sim c_f^+$ and $L_f^-(x)  \sim c_f^-$ as $x \to + \infty$, where
    \begin{equation} \label{eq:cf+--from-c1g-c2g}
        c_f^\pm \doteq \frac{\Gamma(2d)}{2\pi} \left( c_{1,\gamma} \cos( \pi d) \mp  c_{2,\gamma} \sin( \pi d) \right) \in (0,\infty).
    \end{equation}
    \item Suppose that $L_f^+,L_f^-$ are quasi-monotone slowly varying functions at $+ \infty$ 
    % such that $L_f^+(x)  \sim c_f^+$ and $L_f^-(x)  \sim c_f^-$ as $x \to + \infty$, where $c_f^\pm \in (0,\infty)$. 
    Then, Definition \ref{defn:clm-spec} implies Definition \ref{defn:clm-time} with
    \begin{equation} \label{eq:cg1-cg2}
    c_{1,\gamma} \doteq 2\Gamma(1-2d) (c_f^- + c_f^+) \sin(\pi d ), \quad c_{2,\gamma} \doteq 2\Gamma(1-2d) (c_f^- - c_f^+) \cos(\pi d ).
   \end{equation}
\end{enumerate}
\end{proposition}

\subsection{From time to spectral domain } \label{app:subsec:time-to-spec}

\begin{proof}[proof of Proposition \ref{prop:equiv-defn}(i)]
As in the proof of Proposition 2.2.14 in the Appendix of \cite{pipiras_taqqu_2017}, for $\lambda \in [0,\pi) \setminus \{\lambda_0\}$,
\begin{equation}
f_X(\lambda) =  \frac{1}{2\pi} \sum_{h=-\infty}^{\infty} e^{-ih\lambda} \gamma_X(h).
\end{equation}
Then,
\begin{equation} \label{eq:456}
\begin{split}
        f_X(\lambda) &=  \frac{1}{2\pi} \left[ \gamma_X(0) + 2\sum_{h=1}^\infty \cos( h \lambda ) \left(L_{1,\gamma}(h) \cos( \lambda_0 h ) + \xi L_{2,\gamma}(h) \sin( \lambda_0 h ) \right) h^{2d-1} \right] \\ 
    &= \frac{1}{2\pi} \left[ \gamma_X(0) + f_1(\lambda) - \xi  f_2(\lambda) +  f_3(\lambda) + \xi f_4(\lambda) \right] 
\end{split}
\end{equation}
where
\begin{equation} \label{eq:f1-f2-def}
    f_1(\lambda) \doteq \sum_{h=1}^\infty \cos\big((\lambda-\lambda_0) h \big) L_{1,\gamma}(h) h^{2d-1}, \quad f_2(\lambda) \doteq \sum_{h=1}^\infty \sin\big((\lambda-\lambda_0) h \big) L_{2,\gamma(h)} h^{2d-1},
\end{equation}
\begin{equation} \label{eq:f3-f4-def}
    f_3(\lambda) \doteq  \sum_{h=1}^\infty \cos((\lambda + \lambda_0)h  )  L_{1,\gamma}(h)  h^{2d-1}, \quad f_4(\lambda) \doteq  \sum_{h=1}^\infty \sin((\lambda + \lambda_0)h  )  L_{2,\gamma}(h)  h^{2d-1}.
\end{equation}
By Proposition A.2.1 of \cite{pipiras_taqqu_2017}, as $\lambda \to \lambda_0$,
\begin{equation} \label{eq:f1-f2}
\begin{split}
    f_1(\lambda) &\sim |\lambda-\lambda_0|^{-2d} L_{1,\gamma} \left(  \frac{1}{|\lambda - \lambda_0|}  \right) \Gamma(2d) \cos(\pi d), \\
    f_2(\lambda) &\sim \text{sign}(\lambda - \lambda_0) |\lambda-\lambda_0|^{-2d} L_{2,\gamma} \left(  \frac{1}{|\lambda - \lambda_0|}  \right) \Gamma(2d) \sin(\pi d).
\end{split}
\end{equation}

% On the other hand, by using Lagrange's trigonometric identities, for each $N \in \NN$
% \[
% \sum_{h=1}^N \cos((\lambda + \lambda_0)h  ) \le \frac{1}{2} + \frac{1}{2 \min\{ \sin\left(\frac{\lambda_0}{2}\right) ,\sin\left(\frac{\pi + \lambda_0}{2}\right)  \}}, \quad \sum_{h=1}^N \sin((\lambda + \lambda_0)h  ) \le \frac{1}{\min\{ \sin\left(\frac{\lambda_0}{2}\right) ,\sin\left(\frac{\pi + \lambda_0}{2}\right)  \}}.
% \]
% Note that these bounds are uniform in $\lambda$ and that $L_{1,\gamma} h^{2d-1}, L_{2,\gamma} h^{2d-1}$ are eventually decreasing, since $L_{1,\gamma}$ and $L_{2,\gamma}$ belong to the Zygmund class. Therefore, by Dirichlet's test, $f_3(\lambda) \le M, f_4(\lambda) \le M$, for some constant $M$ that does not depend on $\lambda$. 
On the other hand, fix some $0 < \alpha < \lambda_0 < \beta < \pi$, then for $\lambda \in [\alpha-\lambda_0,\beta-\lambda_0]$ we have $\lambda + \lambda_0 \in (0,\pi)$ and that $\max_{\hat \lambda \in [\alpha,\beta]} \{\frac{2}{\sin(\hat \lambda/2)},\frac{2}{\cos(\hat\lambda/2)}\} < \infty$. Moreover, since $L_{1,\gamma},L_{2,\gamma}$ are quasi-monotonic, the display (A.2.6) in Proposition A.2.1 of \cite{pipiras_taqqu_2017} says that, for $\lambda \in [\alpha-\lambda_0,\beta-\lambda_0]$,
\[
f_3(\lambda) \le \max_{\hat \lambda \in [\alpha,\beta]} \frac{2}{\sin(\hat \lambda / 2)} L_{1,\gamma}(1)  (1 + O(1)) < \infty, \quad f_4(\lambda) \le \max_{\hat \lambda \in [\alpha,\beta]} \frac{2}{\cos(\hat \lambda / 2)} L_{1,\gamma}(1) (1 + O(1)) < \infty
\]
where the bounds on the right hand side do not depend on $\lambda$.
By the dominated convergence theorem, as $\lambda \to 0$ (i.e., as $\lambda + \lambda_0 \to \lambda_0 \in [\alpha,\beta]$),
\begin{equation} \label{eq:f3-f4}
\lim_{\lambda \to \lambda_0} f_3(\lambda) =  \sum_{h=1}^\infty \cos(2\lambda_0h  )  L_{1,\gamma}(h)  h^{2d-1} = O(1), \quad \lim_{\lambda \to \lambda_0} f_4(\lambda) =  \sum_{h=1}^\infty \sin( 2 \lambda_0h  )  L_{2,\gamma}(h)  h^{2d-1} = O(1).
\end{equation}
Since $L_{1,\gamma}(x) \to c_{1,\gamma}, \xi L_{2,\gamma}(x) \to c_{2,\gamma}$ as $x \to \infty$, we then get from \eqref{eq:456}, \eqref{eq:f1-f2} and \eqref{eq:f3-f4}, that
\begin{equation} \label{eq:time-to-spec-density}
    f_X(\lambda) \sim \frac{\Gamma(2d)}{2\pi} \left[ c_{1,\gamma} \cos(d\pi) -  \text{sign}(\lambda-\lambda_0) c_{2,\gamma} \sin(d\pi)   \right]    | \lambda - \lambda_0 |^{-2d},
\end{equation}
which confirms the display in \eqref{eq:cf+--from-c1g-c2g}.
\end{proof}

\begin{remark}
    The following relationship holds between $c_f^+,c_f^-$ with $c_\gamma,\phi$ defined in \eqref{rmk-clm-defn-time-equiv}:
        \begin{equation} \label{eq:cfpm-cgamma}
    c_f^\pm = \frac{c_\gamma}{2\pi} \Gamma(2d) \cos(\pi d \mp \phi).
\end{equation}
Indeed, this follows from
\begin{equation}
\begin{split}
    c_{1,\gamma} \cos(\pi d) - \xi \text{sign}(\lambda-\lambda_0) c_{2,\gamma} \sin(\pi d)      
    &=  \cos(\phi) \cos(\pi d) + \text{sign}(\lambda-\lambda_0) \sin(\phi) \sin(\pi d) \\
    &=   c_\gamma \cos(\pi d - \text{sign}(\lambda-\lambda_0)\phi)  .
\end{split}
\end{equation}
\end{remark}

\subsection{From spectral to time domain} \label{app:subsec:spec-to-time}

\begin{proof}[proof of Prop. \ref{prop:equiv-defn}(ii)]
We have
\begin{equation} \label{eq:210}
\begin{split}
\gamma_X(h) &=   2\int_{0}^{\pi} \cos(h\lambda) f_X(\lambda) d\lambda  = 2 \int_0^{\lambda_0} \cos(h\lambda) f_X(\lambda) d\lambda + 2 \int_{\lambda_0}^{\pi} \cos(h\lambda) f_X(\lambda) d\lambda \\
&\doteq 2\left[ \gamma_-(h) + \gamma_+(h)   \right].
\end{split}
\end{equation}
We consider these two quantities separately. First,
\begin{equation}
\begin{split}
    \gamma_-(h) &= \int_0^{\lambda_0} \cos(h \lambda ) L_f^-\left( \frac{1}{\lambda_0 - \lambda}\right) (\lambda_0 - \lambda)^{-2d}   d\lambda \\
    &= \int_0^{\lambda_0} \cos(h (\lambda_0 - \om)) L_f^-\left( \frac{1}{\om} \right) \om^{-2d}   d\om \\
    &= \cos(h \lambda_0) \int_0^{\lambda_0} \cos(h \om)  L_f^-\left( \frac{1}{\om} \right) \om^{-2d}   d\om + \sin(h \lambda_0) \int_0^{\lambda_0} \sin(h \om)  L_f^-\left( \frac{1}{\om} \right) \om^{-2d}   d\om,
\end{split}
\end{equation}
where the second line follows from the change of variables $\lambda_0 - \lambda = \om$. By Proposition A.2.2 of \cite{pipiras_taqqu_2017} and since $L_f^-$ is quasi-monotone, we have that
\begin{equation}
    \int_0^{\lambda_0} \cos(h \om)  L_f^-\left( \frac{1}{\om} \right) \om^{-2d}   d\om \sim h^{2d-1} L_f^-(h) \Gamma(1-2d) \sin(\pi d),
\end{equation}
and similarly
\begin{equation}
    \int_0^{\lambda_0} \sin(h \om)  L_f^-\left( \frac{1}{\om} \right) \om^{-2d}   d\om  \sim h^{2d-1} L_f^-(h) \Gamma(1-2d) \cos(\pi d).
\end{equation}
Analogous calculations show that
\begin{equation} \label{eq:spec-to-time-gamma+}
\begin{split}
    \gamma_+(h) &= \int_{\lambda_0}^\pi \cos(h \lambda ) L_f^+\left( \frac{1}{\lambda - \lambda_0}\right) ( \lambda - \lambda_0)^{-2d}   d\lambda \\
    &= \int_0^{\pi - \lambda_0} \cos(h (\lambda_0 + \om)) L_f^+\left( \frac{1}{\om} \right) \om^{-2d}   d\om \\
    &= \cos(h \lambda_0) \int_0^{\pi - \lambda_0} \cos(h \om)  L_f^+\left( \frac{1}{\om} \right) \om^{-2d}   d\om - \sin(h \lambda_0) \int_0^{\pi - \lambda_0} \sin(h \om)  L_f^+\left( \frac{1}{\om} \right) \om^{-2d}   d\om,
\end{split}
\end{equation}
where
\begin{equation}
    \int_0^{\pi - \lambda_0} \cos(h \om)  L_f^+\left( \frac{1}{\om} \right) \om^{-2d}   d\om \sim h^{2d-1} L_f^+(h) \Gamma(1-2d) \sin\left( \pi d   \right),
\end{equation}
and
\begin{equation}
    \int_0^{\pi - \lambda_0} \sin(h \om)  L_f^+\left( \frac{1}{\om} \right) \om^{-2d}   d\om  \sim h^{2d-1} L_f^+(h) \Gamma(1-2d) \cos\left( \pi d   \right).
\end{equation}
Since $L_f^{\pm}(h) \to c_f^{\pm}$ as $h \to \infty$, \eqref{eq:210} can be written as
\begin{equation}
\begin{split}
    \gamma_X(h) &= \cos(h \lambda_0) \left[ h^{2d-1} c_f^- 2 \Gamma(1-2d) \sin(\pi d)  +R_1^-(h)) \right] \\
    &\quad+ \sin(h \lambda_0) \left[ h^{2d-1} c_f^- 2 \Gamma(1-2d) \cos(\pi d)  + R_2^-(h)) \right] \\
    &\quad + \cos(h \lambda_0) \left[ h^{2d-1} c_f^+ 2 \Gamma(1-2d) \sin(\pi d)  + R_1^+(h)) \right] \\
    &\quad- \sin(h \lambda_0) \left[ h^{2d-1} c_f^+ 2 \Gamma(1-2d) \cos(\pi d)  + R_2^+(h)) \right],
\end{split}
\end{equation}
where $R_{1}^\pm(h) \doteq 2(L_f^\pm(h) - c_f^{\pm}) \Gamma(1-2d) \sin(\pi d) h^{2d-1} = o(h^{2d-1})$ and $R_{2}^\pm(h) \doteq 2(L_f^\pm(h) - c_f^{\pm}) \Gamma(1-2d) \cos(\pi d) h^{2d-1} = o(h^{2d-1})$. By defining $c_{1,\gamma},c_{2,\gamma}$ as in \eqref{eq:cgamma-psi}, we thus have that
\begin{equation} \label{eq:213}
\begin{split}
    \gamma_X(h) &= 2 \Gamma(1-2d) h^{2d-1}  \left[(c_f^+ + c_f^-)  \sin(\pi d) \cos(\lambda_0 h) + (c_f^- - c_f^+)  \cos(\pi d) \sin(\lambda_0h)\right] + R(h) \\
    &= c_{1,\gamma} \cos(\lambda_0 h) h^{2d-1}  + c_{2,\gamma} \sin(\lambda_0 h) h^{2d-1} + R(h),
\end{split}
\end{equation}
where 
\begin{equation} \label{eq:spec-to-time-R}
\begin{split}
R(h) &\doteq \cos(h \lambda_0) R_1^-(h) + \sin(h \lambda_0) R_2^-(h) + \cos(h \lambda_0) R_1^+(h) - \sin(h \lambda_0) R_2^+(h) \\
&= \cos(\lambda_0 h) o(h^{2d-1}) + \sin(\lambda_0 h) o(h^{2d-1}).
\end{split} 
\end{equation}
This concludes the proof.
\end{proof}

\begin{remark} \label{rmk:cg-c1g-c2g}
    Note that \eqref{eq:213} can be reformulated as in remark \ref{rmk-clm-defn-time-equiv} by writing
    \begin{equation}
        \gamma_X(h) =  c_\gamma \cos(\lambda_0 h + \phi) h^{2d-1} + R(h),
    \end{equation}
    where $R(h)$ is given in \eqref{eq:spec-to-time-R}, and the constants $\phi$ and $c_\gamma$ are given by
    \begin{equation} \label{eq:cgamma-psi}
   \begin{split}
    c_\gamma &\doteq 2\Gamma(1-2d) \sqrt{(c_f^+ + c_f^-)^2 \left(\sin(\pi d )\right)^2 + (c_f^+ - c_f^-)^2 \left(\cos(\pi d ) \right)^2} \\
    &= 2\Gamma(1-2d)\sqrt{(c_f^+)^2 + (c_f^-)^2 - 2 c_f^+ c_f^-\left(\cos( 2 \pi d) \right)^2}, \\
    \phi &\doteq  \arcsin \left( \frac{(c_f^+ - c_f^-) \cos(\pi d)}{\sqrt{(c_f^+)^2 + (c_f^-)^2 - 2 c_f^+ c_f^-\left(\cos(2 \pi d) \right)^2}}  \right) .
   \end{split}
\end{equation}
\end{remark}

\subsection{Set of admissible cyclical phases and special cases}
\label{subsubsec:admis-phase}

Since $c_f^+,c_f^- > 0$, note that \eqref{eq:cfpm-cgamma} yields
\[
-\frac{\pi}{2} < d\pi - \phi < \frac{\pi}{2}, -\frac{\pi}{2} <  \phi - d\pi < \frac{\pi}{2}
\]
so that, as stated in \eqref{eq:admiss-sets-def},
\[
\phi \in \overset{\circ}{\cli_d} \doteq \left(\left(d - \frac{1}{2} \right)\pi  , \left(\frac{1}{2} - d\right) \pi \right).
\]
When $c_f^+ = c_f^- = c_f$ (symmetric case), we have, from Proposition \ref{prop:equiv-defn},
\begin{equation} \label{eq:cf-cf+cf}
c_{1,\gamma} = 4 \Gamma(1-2d) c_f \sin(\pi d), \quad c_{2,\gamma} = 0
\end{equation}
or, in terms of $c_\gamma,\phi$,
\[
c_\gamma = 2 \sqrt{2} \Gamma(1-2d) c_f \sin(2 \pi d), \quad \phi = 0.
\]
The case $c_f^\pm = 0$, or $\phi = \pm \left(\frac{1}{2} - d\right) \pi$, is more delicate and not covered by Proposition \ref{prop:equiv-defn}. A deeper analysis will be pursued in the next Appendix, but we list here some elementary observations. Note that if, e.g., $c_f^+ = 0$, then Proposition \ref{prop:equiv-defn} suggests (in a limiting sense, as $c_f^+ \to 0$) that
\[
c_{1,\gamma} = 2 \Gamma(1-2d) c_f^- \sin(\pi d), \quad c_{2,\gamma} = 2 \Gamma(1-2d) c_f^- \cos(\pi d), \quad \frac{c_{1,\gamma}}{c_{2,\gamma}} =  \tan(\pi d),
\]
or equivalently,
\[
c_\gamma = 2 \Gamma(1-2d) c_f^-, \quad \phi =  \left(d - \frac{1}{2}\right) \pi.
\]
Similarly, $c_f^- = 0$ corresponds to
\[
c_{1,\gamma} = 2 \Gamma(1-2d) c_f^+ \sin(\pi d), \quad c_{2,\gamma} = - 2 \Gamma(1-2d) c_f^+ \cos(\pi d), \quad \frac{c_{1,\gamma}}{c_{2,\gamma}} = - \tan(\pi d),
\]
or equivalently
\[
c_\gamma = 2 \Gamma(1-2d) c_f^+, \quad \phi =  \left( \frac{1}{2} - d\right) \pi.
\]

% As in \eqref{eq:cf-0} and \eqref{eq:cf+0}, note again that the boundary values $\phi = \pm \left(\frac{1}{2}-d\right) \pi$ correspond to $c_f^\mp = 0$.

% When, e.g., $c_f^+ > 0$ and $c_f^- = 0$, we get that
% \begin{equation} \label{eq:cf-0}
%     c_\gamma = 2 \Gamma(1-2d) c_f^+, \quad \phi =  \left( \frac{1}{2} - d \right) \pi.
% \end{equation}
% When $c_f^- > 0$ and $c_f^+ = 0$, we get that
% \begin{equation} \label{eq:cf+0}
%     c_\gamma = 2 \Gamma(1-2d) c_f^-, \quad \phi = - \left( \frac{1}{2} - d \right) \pi.
% \end{equation}

\section{Definitions of CLM in the ``boundary" case} \label{App:subsec-boundary}

As anticipated, the ``boundary" case $\frac{c_{1,\gamma}}{c_{2,\gamma}} = \pm \tan(\pi d)$, or equivalently $ \phi = \mp  \left( \frac{1}{2} - d \right) \pi$, requires special treatment, and we provide here a few results sheding light into its representation in the time spectral domains. We first provide a definition for the ``boundary" case (Definition \ref{defn:clm-time}). 

\begin{defn}(Time domain, CLM in the ``boundary" case) \label{defn:clm-time-bound}
 We say that $\{X_n\}_{n \in \ZZ}$ exhibits CLM in the ``boundary" case if its ACVF satisfies
        \begin{equation} \label{eq:def-eq-acvf-boundary}
        \gamma_X(h) = c_\gamma \cos(\lambda_0 h + \phi) h^{2d-1} + L_{1,\gamma}(h) \cos(\lambda_0 h) h^{2\delta-1} + \xi L_{2,\gamma}(h) \sin(\lambda_0 h) h^{2\delta-1} , \quad h \in \ZZ,
    \end{equation}
     where $\lambda_0 \in (0,\pi), \xi = \pm 1, \phi = \pm  \left( \frac{1}{2} - d \right) \pi$, and $-\infty < \delta < d < \frac{1}{2}$ are constants, and $L_{1,\gamma}, L_{2,\gamma} : \RR \to (0,\infty)$ are slowly varying, symmetric functions around $0$ with $L_{1,\gamma}(x) \sim c_{1,\gamma} \in (0,\infty)$ and $\xi L_{2,\gamma}(x) \sim c_{2,\gamma} \in \RR$ as $x \to \infty$ (here $\xi =\text{sign}(c_{2,\gamma})$) and, moreover,
    \begin{equation} \label{eq:789}
    c_{1,\gamma} \in \RR_+ \; \text{and} \; c_{2,\gamma} = 0, \quad \text{or} \quad 
    \frac{c_{1,\gamma}}{c_{2,\gamma}} \in [-\tan(\pi \delta), \tan(\pi \delta)].
    \end{equation}
    % \item \label{defn:clm-time-bound-II}  We say that $\{X_n\}_{n \in \ZZ}$ exhibits CLM in the ``boundary" case \textit{of type II} (or, simply, is of type II) if its ACVF satisfies
    % \begin{equation}
    %    \gamma_X(h) = L_{1,\gamma}(h) \cos(\lambda_0 h+ \phi) h^{2d-1} + \cos(\lambda_0 h) O(h^{2\delta-1}) + \sin(\lambda_0 h) O(h^{2\delta-1}),
    % \end{equation}
    % where $\lambda_0 \in (0,\pi), \phi = \pm\left( \frac{1}{2} - d \right), 0 \le \delta < d < \frac{1}{2}$ and $L_{1,\gamma} : \RR \to (0,\infty)$ is a slowly varying, symmetric function around $0$ with $L_{1,\gamma}(x) \sim c_{1,\gamma} \in (0,\infty)$ as $x \to \infty$.
    % \end{enumerate} 
\end{defn}

We now define the expected spectral representation of a series exhibiting CLM in the ``boundary" case.

% \begin{remark}
%     We remark that in \eqref{eq:789} above, we take the ratio of $\frac{c_{1,\gamma}}{c_{2,\gamma}}$ to belong to the open interval. Indeed, taking $\frac{c_{1,\gamma}}{c_{2,\gamma}} = \pm \tan(\pi \delta)$ corresponds to the ``boundary" case for the second-order asymptotics and so they can be neglected below.
% \end{remark}

\begin{defn}(Spectral domain, CLM with asymmetric memory case) \label{defn:clm-spec-assym}
    A second-order stationary time series $\{X_n\}_{n \in \ZZ}$ is said to exhibit CLM with asymmetric memory if its spectral density satisfies
\begin{equation} \label{eq:spec-rigorous-defn-bound}
    f_X(\lambda) = \begin{cases}
        L_f^- \left(\frac{1}{\lambda_0 - \lambda}\right)  (\lambda_0 - \lambda)^{-2d_-}, & 0 < \lambda < \lambda_0, \vspace{3mm}\\
        L_f^+ \left(\frac{1}{\lambda - \lambda_0}\right)  (\lambda - \lambda_0)^{-2d_+}, & \lambda_0 < \lambda < \pi,
    \end{cases}
\end{equation}
where $0 \le \min\{d_-,d_+\} < \max\{d_-,d_+\} < \frac{1}{2} $, and $L_f^-: \left(\frac{1}{\lambda_0},\infty\right) \to (0,\infty)$, $L_f^+: \left(\frac{1}{\pi - \lambda_0},\infty\right) \to (0,\infty)$ are two slowly varying functions at $\infty$.
\end{defn}

\begin{remark}
    Note that in Definition \ref{eq:spec-rigorous-defn-bound}, a particularly important case is when $L_f^+(x) \sim c_f^+ ,L_f^-(x) \sim c_f^-$ as $x \to \infty$ for some constants $c_f^\pm \in \RR_+$. However, we do not require this in the definition, to allow for, e.g., the case $L_f^\pm(x) \sim \log(x)$. Indeed, such slowly varying functions can arise when we obtain CLM with asymmetric memory from from CLM in the ``boundary" case (see, e.g., Proposition \ref{prop:equiv-defn-boundary}\eqref{it:time-to-spec-0-delta-border-2} below).
\end{remark}

Next is a result obtaining CLM with asymmetric memory in the spectral domain from series exhibiting CLM in the ``boundary" case (i.e., obtaining Definition \ref{defn:clm-spec-assym} from Definition \ref{defn:clm-time-bound}). Without loss of generality, we can restrict our investigation to the case $\phi =  \left( \frac{1}{2} -d \right) \pi$, which is expected to correspond to $c_f^- = 0$ (see the discussion of Section \ref{subsubsec:admis-phase}). An analogous (but symmetric) statement can be easily stated for $\phi = - \left( \frac{1}{2} -d \right) \pi$.

\begin{proposition} \label{prop:equiv-defn-boundary}
Suppose that $L_{1,\gamma}, L_{2,\gamma}$ are slowly varying functions at $+ \infty$ that belong to the Zygmund class. Then, Definition \ref{defn:clm-time-bound} with $\phi =  \left( \frac{1}{2} -d \right) \pi$ and 
    \[
    c_{1,\gamma} \in (0,\infty), \; \text{and} 
    \; c_{2,\gamma} = 0 \quad \text{or} \quad \frac{c_{1,\gamma}}{c_{2,\gamma}} \in (-\tan(\pi \delta), \tan(\pi \delta)]
    \]
    implies Definition \ref{defn:clm-spec-assym} with $d_+ = d$,  
    \begin{equation} \label{prop:time-to-spec-bound-cf+}
        L_f^+(x)  \sim c_f^+  \doteq \sin(2\pi d) \frac{c_\gamma}{2\pi},\quad \text{as } x \to + \infty,
    \end{equation}
    and:
    \begin{enumerate}[(i)]
        \item \label{it:time-to-spec-0-delta-border} If $0< \delta < d < \frac{1}{2}$, then $d_- = \delta$ and $ L_f^-(x)  \sim c_f^-$ as $x \to +\infty$, where
        \begin{equation}
            c_f^- \doteq \frac{\Gamma(2\delta)}{2\pi} \left[ c_{1,\gamma} \cos(\delta\pi) + c_{2,\gamma} \sin(\delta\pi)   \right] \in (0,\infty).
        \end{equation}
        \item \label{it:time-to-spec-0-delta-border-2} 
       If $0 = \delta < d < \frac{1}{2}$, then $d_- = 0$ and $L_f^-$ is given by:
        \begin{equation}
            L_f^-(x) \doteq O(1) +  \frac{1}{2\pi} \sum_{h=1}^\infty \frac{L_{1,\gamma}(h)}{h} \cos\left(\frac{h}{x}\right).
        \end{equation}
        In particular, $L_f^-$ is slowly varying at $+ \infty$ since, as $x \to \infty$,
        \begin{equation}
            L_f^-(x) \sim \frac{c_{1,\gamma}}{2\pi}  \log x.
        \end{equation}
        \item \label{it:time-to-spec-0-delta-border-3}  If $-\infty < \delta < 0 < d < \frac{1}{2}$, then $d_- = 0$, and $ L_f^-(x)  \sim c_f^-$ as $x \to +\infty$, where $c_f^-$ is a constant defined in \eqref{eq:cf^-c1c2c3} below.
    \end{enumerate}
\end{proposition}

\begin{proof}
Note that we can write, for $h \in \ZZ$,
\begin{equation}
\gamma_X(h) = c_\gamma \cos(\lambda_0 h + \phi) h^{2d-1} + L_{1,\gamma}(h) \cos(\lambda_0 h) h^{2\delta-1} + \xi L_{2,\gamma}(h) \sin(\lambda_0 h) h^{2\delta-1} = \gamma_1(h) + \gamma_2(h),
\end{equation}
with
\begin{equation} 
\gamma_1(h) \doteq  c_\gamma \cos(\lambda_0 h + \phi) h^{2d-1}, \quad \gamma_2(h) \doteq L_{1,\gamma}(h) \cos(\lambda_0 h) h^{2\delta-1} + \xi L_{2,\gamma}(h) \sin(\lambda_0 h) h^{2\delta-1}.
\end{equation}
Calculations similar to \eqref{eq:456}--\eqref{eq:time-to-spec-density} illustrate that, as $\lambda \to \lambda_0^-$,
\begin{equation} \label{eq:time-spec-boundary-100}
\begin{split}
  \sum_{h=-\infty}^\infty e^{-ih\lambda} \gamma_{1}(h) &= \frac{1}{2\pi} \bigg[ \gamma_1(0) + c_\gamma \sin(d\pi) \sum_{h=1}^\infty \cos((\lambda - \lambda_0) h) h^{2d-1} + \cos(d \pi) \sum_{h=1}^\infty \sin((\lambda_0 - \lambda) h) h^{2d-1}\bigg. \\
  &\quad+ \bigg. \sin(d\pi) c_\gamma \sum_{h=1}^\infty \cos((\lambda + \lambda_0) h) h^{2d-1} - \cos(d\pi) c_\gamma \sum_{h=1}^\infty \sin((\lambda + \lambda_0) h) h^{2d-1} \bigg]  \\
&\sim \frac{1}{2\pi}\left( \gamma_1(0)  + \sin(d\pi) c_\gamma \sum_{h=1}^\infty \cos(2\lambda_0 h) h^{2d-1} - \cos(d\pi) c_\gamma \sum_{h=1}^\infty \sin(2 \lambda_0 h) h^{2d-1}\right)\\
& \doteq c_1 ,
\end{split}
\end{equation}
where we have used the facts that $\phi = \left( \frac{1}{2} - d \right) \pi$ in the first equality, and Lemma \ref{lemma:second-order-time-to-spec} and that the series in the last display converge by Dirichlet's test in the second to last line. On the other hand, as $\lambda \to \lambda_0^+$,
\begin{equation} \label{eq:time-spec-boundary-101}
\begin{split}
    \sum_{h=-\infty}^\infty e^{-ih\lambda} \gamma_{1}(h) &= \left[ \cos(\phi) \cos(\pi d) - \text{sign}(\lambda - \lambda_0) \sin(\phi) \sin(\pi d) \right]  c_\gamma \frac{1}{2\pi} |\lambda - \lambda_0|^{-2d} + O(1) \\
    &= \sin(2 d \pi)  \frac{c_\gamma}{2\pi} |\lambda - \lambda_0|^{-2d} + O(1),
\end{split}
\end{equation}
which, since $\delta < d$, gives \eqref{prop:time-to-spec-bound-cf+}. We now investigate the spectral density corresponding to $\gamma_2$. In the case $0 < \delta < d < \frac{1}{2}$, calculations identical to the ones of Section \ref{app:subsec:time-to-spec}, as $\lambda \to \lambda_0$,
\begin{equation} \label{eq:time-spec-boundary-102}
\sum_{h=-\infty}^\infty e^{-ih\lambda} \gamma_{2} (h) \sim \frac{\Gamma(2\delta)}{2\pi} \left[ c_{1,\gamma} \cos(\delta\pi) - \text{sign}(\lambda-\lambda_0) c_{2,\gamma} \sin(\delta\pi)   \right] |\lambda - \lambda_0|^{-2\delta}.
\end{equation}
The displays in \eqref{eq:time-spec-boundary-100}, \eqref{eq:time-spec-boundary-101}, \eqref{eq:time-spec-boundary-102} say that, in this case, the leading order dynamics are given by
\[
f_X(\lambda) \sim \begin{cases}
    \frac{\Gamma(2\delta)}{2\pi} \left[ c_{1,\gamma} \cos(\delta\pi) + c_{2,\gamma} \sin(\delta\pi)   \right] |\lambda - \lambda_0|^{-2\delta} & \lambda \to \lambda_0^-, \\
    \sin(2\pi d) \frac{c_\gamma}{2\pi} |\lambda - \lambda_0|^{-2d} &  \lambda \to \lambda_0^+.
\end{cases}
\]
This concludes the proof of \eqref{it:time-to-spec-0-delta-border}.

% \footnote{Note that, in the terminology of \cite{bingham_goldie_teugels_1987}, the results of Zygmund hold for slowly varying functions in the Zygmund class.\cite{bingham_goldie_teugels_1987} presents the result for sines in Section 4.3, but I cannot find the one for cosines there, so I will cite the book of Zygmund instead} 
Now we turn to the case $\delta = 0$. 
From the calculations in \eqref{eq:456}--\eqref{eq:time-to-spec-density}, 
\begin{equation} \label{eq:time-spec-boundary-108}
\sum_{h=-\infty}^\infty e^{-ih\lambda} \gamma_{2} (h) = \frac{1}{2\pi} \left[ \gamma_{2}(0) + f_1(\lambda) - \xi  f_2(\lambda) +  f_3(\lambda) + \xi f_4(\lambda) \right],
\end{equation}
where $f_i(\lambda),i=1,\dots,4$ were defined in \eqref{eq:f1-f2-def} (with $d$ replaced by $\delta$) and \eqref{eq:f3-f4-def}, and $f_3(\lambda), f_4(\lambda) = O(1)$. We now estimate $f_1(\lambda),f_2(\lambda)$.

Since $L_{1,\gamma}(x) \sim c_{1,\gamma} \in (0,\infty)$  we have that,
\[
\sum_{h=1}^\infty \frac{L_{1,\gamma}(h)}{h} = \infty \quad \text{and} \quad \int_1^{1/\lambda} \frac{L_{1,\gamma}(u)}{u} du \sim - c_{1,\gamma}  \log (\lambda) \quad \text{as } \lambda \to 0^+.
\]
Upon recalling that $L_{1,\gamma}$ is slowly varying function in the Zygmund class, Theorem 5.2.15 of \cite{zygmund_2003} and the display above say that, as $\lambda \to \lambda_0^-$ 
\begin{equation} \label{eq:Lf_-boundary}
    f_1(\lambda) = \sum_{h=1}^\infty \frac{L_{1,\gamma}(h)}{h} \cos(h (\lambda_0 -\lambda)) \sim - c_{1,\gamma}  \log (\lambda_0 - \lambda).
\end{equation}
In particular, $L_f^-(x)$ is a slowly varying function. In addition, $\xi L_{2,\gamma}(x) \sim c_{2,\gamma} \in \RR$ as $x \to \infty$ and $L_{2,\gamma}$ is in the Zygmund class. From Theorem 5.2.6 and remark (2.13) of \cite{zygmund_2003}, as $\lambda \to \lambda_0^+$
\begin{equation} \label{eq:f2-bound-finite}
    f_2(\lambda) = \sum_{h=1}^\infty \frac{L_{2,\gamma}(h)}{h} \sin(h (\lambda_0 -\lambda)) \sim \frac{1}{2} \pi L_{2,\gamma}\left(\frac{1}{\lambda_0 - \lambda}\right) \sim \frac{c_{2,\gamma}}{2}\pi  = O(1).
\end{equation}
In view of \eqref{eq:time-spec-boundary-100}, \eqref{eq:time-spec-boundary-101},  \eqref{eq:time-spec-boundary-108}, \eqref{eq:time-spec-boundary-108}, \eqref{eq:Lf_-boundary}, and \eqref{eq:f2-bound-finite}
\[
f_X(\lambda) \sim \begin{cases}
   - \frac{c_{1,\gamma}}{2\pi}  \log \left(\lambda_0 - \lambda \right)  & \lambda \to \lambda_0^-, \\
    \sin(2\pi d) \frac{c_\gamma}{2\pi} (\lambda - \lambda_0)^{-2d} &  \lambda \to \lambda_0^+,
\end{cases}
\]
confirming \eqref{it:time-to-spec-0-delta-border-2}.

Finally, let $-\infty < \delta < 0 < d < \frac{1}{2}$ and note that the identity in \eqref{eq:time-spec-boundary-108} is still true. From Theorem 4.3.2 of \cite{bingham_goldie_teugels_1987} (with $\mu = 1 - 2\delta \in (1,2)$) and the discussion at the end of the section in the same reference, we have as $\lambda \to 0^+$
\[
f_2(\lambda) = o(1).
\]
Moreover, by DCT, as $\lambda \to 0^+$
\begin{equation} \label{eq:c2-def}
    f_1(\lambda) \sim \sum_{h=1}^\infty \frac{L_{1,\gamma}(h)}{h^{1-2\delta}} \doteq c_2,
\end{equation}
where the convergence of the series follows by, e.g., Proposition 1.5.10 of \cite{bingham_goldie_teugels_1987} and the integral test since $\frac{L_{1,\gamma}(h)}{h^{1-2\delta}}$ is ultimately decreasing from the Zygmund property of $L_{1,\gamma}$. Finally, Dirichlet's test shows that, once again, as $\lambda \to \lambda_0^+$
\begin{equation} \label{eq:c3-def}
    f_3(\lambda) + \xi f_4(\lambda) \sim \sum_{h=1}^\infty \cos(2\lambda_0 h) L_{1,\gamma}(h) h^{2\delta -1} + \xi \sum_{h=1}^\infty \sin(2\lambda_0 h) L_{2,\gamma}(h) h^{2\delta -1} \doteq c_3 < \infty,
\end{equation}
Now define
\begin{equation} \label{eq:cf^-c1c2c3}
    c_f^- \doteq c_1 + \frac{1}{2\pi}\left( \gamma_{2}(0) + c_2 + c_3 \right),
\end{equation}
where $c_i,i=1,2,3$ are defined in \ref{eq:time-spec-boundary-100}, \eqref{eq:c2-def}, and \eqref{eq:c3-def} respectively. This leads to 
\[
f_X(\lambda) \sim \begin{cases}
    c_f^- & \lambda \to \lambda_0^-, \\
    \sin(2\pi d) \frac{c_\gamma}{2\pi} |\lambda - \lambda_0|^{-2d} &  \lambda \to \lambda_0^+,
\end{cases}
\]
which concludes the proof.
\end{proof}

The following proposition provides some conditions under which the ``boundary" case of CLM can be obtained from CLM with asymmetric memory.

\begin{proposition}     \label{it:spec-to-time-border} 
Suppose that $L_f^+(x) \doteq c_f^+ + \tilde L_f^+(x) x^{-\veps}$, where $\veps \in (0,2d_+)$, and that $\tilde L_f^+(x)$ is quasi-monotone and slowly varying at $+ \infty$ with $\tilde L_f^+(x)  \sim \tilde c_f^+ \in (0,\infty)$ as $x \to \infty$. Let, moreover, one of the following three conditions hold:
\begin{enumerate}[(i)]
    \item \label{prop:item-spec-to-time-bound-1} $0 < d_- < d_+$ and $L_{f}^-(x) \sim c_f^- \in (0,\infty)$ as $x \to \infty$,
        
     \item \label{prop:item-spec-to-time-bound-2} $d_- = 0$, $L_{f}^-(x)$ is non-increasing,  and $\lim_{x \to \infty} L_{f}^-(x) = c \in [0,\infty)$, or
        
    \item \label{prop:item-spec-to-time-bound-3} $d_- = 0 $, $L_{f}^-(x)$ is differentiable, and $(L_{f}^-)'(x)$ is uniformly bounded in $\left(\frac{1}{\lambda_0},\infty\right)$. 
    \end{enumerate}
Then, Definition \ref{defn:clm-spec-assym} implies Definition \ref{defn:clm-time-bound} with 
     \begin{equation} \label{eq:phi-cgamma-boun-spec-to-time}
     d \doteq d_+, \quad \phi \doteq \left( \frac{1}{2} - d \right) \pi,  \quad c_\gamma \doteq 2 \Gamma(1-2d_+) c_f^+, \quad \delta \doteq \max \{d_-,d_+ - \veps / 2\},
   \end{equation}
  \begin{equation} \label{eq:L1g-spec-to-time}
    c_{1,\gamma}(x) = \begin{cases}
      2 \Gamma(1-2d_-)  \sin(\pi d_-) c_f^- & \veps > 2(d_+ - d_-), \\
      2 \Gamma(1-2d_-)  \sin(\pi d_-) c_f^- +  2 \Gamma(1-2d_+ + \veps)  \sin(\pi (d_+ - \veps /2) ) \tilde c_f^+ & \veps = 2(d_+ - d_-), \\
       2 \Gamma(1-2d_+ + \veps)  \sin(\pi (d_+ - \veps /2) ) \tilde c_f^+  & \veps < 2(d_+ - d_-),
    \end{cases}
\end{equation} 
and 
\begin{equation} \label{eq:L2g-spec-to-time}
    c_{2,\gamma}(x) = \begin{cases}
      2 \Gamma(1-2d_-)  \cos(\pi d_-) c_f^- & \veps > 2(d_+ - d_-), \\
      2 \Gamma(1-2d_-)  \cos(\pi d_-) c_f^- +  2 \Gamma(1-2d_+ + \veps)  \sin(\pi (d_+ - \veps /2) ) \tilde c_f^+ & \veps = 2(d_+ - d_-), \\
       - 2 \Gamma(1-2d_+ + \veps)  \cos(\pi (d_+ - \veps /2) ) \tilde c_f^+  & \veps < 2(d_+ - d_-).
    \end{cases}
\end{equation}
% is quasi-monotone, where $\veps \in [0,1-2d)$ and $\tilde L_f^+(x)$ is slowly-varying at $+\infty$ (in particular, $L_f^+(x)  \sim c_f^+ \in (0,\infty)$ as $x \to + \infty$ and so is slowly varying at $+ \infty$). 
% Then, Definition \ref{defn:clm-spec-assym} implies Definition \ref{defn:clm-time-bound} with $\delta = \max \{d_-,d_+ - \veps / 2\}$ and 
%      \begin{equation} \label{eq:phi-cgamma-boun-spec-to-time}
%      \phi \doteq \left( \frac{1}{2} - d \right) \pi, \quad L_{1,\gamma}(x) \doteq 2 \Gamma(1-2d) L_f^+(x) \sim 2 \Gamma(1-2d) c_f^+, \quad \text{as } x \to \infty.
%    \end{equation}
% \[
% \cos(\lambda_0 h) O(h^{2\delta-1}) + \sin(\lambda_0 h) O(h^{2\delta-1}) = L_{2,\gamma}(h) \cos(\lambda_0 h - \phi) h^{2\delta-1} + \cos(\lambda_ 0 ) o(h^{2d-1}) + \sin(\lambda_0 h) o(h^{2d-1}),
% \]
% where
%     \begin{equation}
%             L_{2,\gamma}(x) \doteq 2\Gamma(1-2\delta) L_f^-(x)  \sim 2\Gamma(1-2\delta) c_f^- , \quad \text{as } x \to \infty.
%     \end{equation}
\end{proposition}

\begin{proof}
We start with an a priori estimate. Recall the display in \eqref{eq:210}. In view of \eqref{eq:spec-to-time-gamma+}, the form of $L_f^+$ in the assumption, and Remark \ref{rmk:cg-c1g-c2g}, we write
\begin{equation} \label{eq:bound-g+}
\begin{split}
   2\gamma_+(h) &= 2\cos(h \lambda_0) \int_0^{\pi - \lambda_0} \cos(h  \om ) L_{f}^+\left(\frac{1}{\om}\right) \om^{-2d_+} d\om - 2\sin(h \lambda_0) \int_0^{\pi - \lambda_0} \sin(h  \om ) L_{f}^+\left(\frac{1}{\om}\right) \om^{-2d_+} d\om \\
   &= 2 c_f^+ \cos(h \lambda_0) \int_0^{\pi - \lambda_0} \cos(h  \om ) \om^{-2d_+ } d\om - 2 c_f^+ \sin(h \lambda_0) \int_0^{\pi - \lambda_0} \sin(h  \om )  \om^{-2d_+} d\om \\
   &\quad + 2 \cos(h \lambda_0) \int_0^{\pi - \lambda_0} \cos(h  \om ) \tilde L_{f}^+\left(\frac{1}{\om}\right) \om^{-2d_+ + \veps} d\om \\
   &\quad- 2\sin(h \lambda_0) \int_0^{\pi - \lambda_0} \sin(h  \om ) \tilde L_{f}^+\left(\frac{1}{\om}\right) \om^{-2d_+ + \veps} d\om \\
   &= c_\gamma \cos(\lambda_0 h + \phi) h^{2d_+-1} \\
   &\quad+ 2 \Gamma(1-2d_+ + \veps) \sin((d_+ - \veps/2) \pi) \tilde L_{f}^+\left(h \right) \cos(\lambda_0 h) h^{2d_+-1 - \veps} \\
   &\quad-  2 \Gamma(1-2d_+ + \veps) \cos((d_+ - \veps/2) \pi) \tilde L_{f}^+\left(h \right) \sin(\lambda_0 h) h^{2d_+-1 - \veps} + o(h^{2d_+-1 - \veps}) 
\end{split}
\end{equation}
where the third equality follows from Lemma \ref{lemma-second-order-spec-to-time} and Proposition A.2.2 of \cite{pipiras_taqqu_2017} since $-2d_+ + \veps < 0$, and
$d_+,\phi,c_\gamma$ were defined in \eqref{eq:phi-cgamma-boun-spec-to-time}.

Now we consider different cases for the values of $d_-$. If $0 < d_- < d_+$, from Proposition A.2.2 of \cite{pipiras_taqqu_2017},
\begin{equation} \label{eq:bound-g-}
\begin{split}
2\gamma_-(h) &= 2\cos(h \lambda_0) \int_0^{\lambda_0} \cos(h \lambda ) L_{f}^-\left( \frac{1}{\om} \right) \om^{-2 d_-} d\om + 2\sin(h \lambda_0) \int_0^{\lambda_0} \sin(h \om )  L_{f}^-\left( \frac{1}{\om} \right) \om^{-2d_-} d\om  \\
    &\sim 2\Gamma(1-2d_-) L_{f}^-(h) (\cos(\pi d_-) \sin(h \lambda_0 )+ \sin(\pi d_-) \cos(h \lambda_0) ) h^{2d_--1}.
\end{split}
\end{equation}
Combining \eqref{eq:210}, \eqref{eq:bound-g+}, and \eqref{eq:bound-g-}, and from the definition of $\delta$ in \eqref{eq:phi-cgamma-boun-spec-to-time}, we write
\begin{equation}
\begin{split}
    \gamma_X(h) &= 2 \gamma_{+}(h) + 2 \gamma_-(h) \\
    &= c_\gamma \cos(\lambda_0 h + \phi) h^{2d_+-1} \\
    &\quad+ 2 \Gamma(1-2d_+ + \veps) \sin((d_+ - \veps/2) \pi) \tilde L_{f}^+\left(h \right) \cos(\lambda_0 h) h^{2d_+-1 - \veps} \\
   &\quad-  2 \Gamma(1-2d_+ + \veps) \cos((d_+ - \veps/2) \pi) \tilde L_{f}^+\left(h \right) \sin(\lambda_0 h) h^{2d_+-1 - \veps} \\
    &\quad+ 2\Gamma(1-2d_-) L_{f}^-(h) (\cos(\pi d_-) \sin(h \lambda_0 )+ \sin(\pi d_-) \cos(h \lambda_0) ) h^{2d_--1}
     \\
    &\quad   + o(h^{2d_+-1 - \veps}) + (\cos(\lambda_0 h) + \sin(\lambda_0 h) )O(h^{-1}) \\
    &=   c_\gamma \cos(\lambda_0 h + \phi) h^{2d-1} + L_{1,\gamma}(h) \cos(\lambda_0 h) h^{2\delta -1}   +  \xi L_{2,\gamma}(h) \sin(\lambda_0 h)) h^{2\delta -1}, 
\end{split}
\end{equation}
where $L_{1,\gamma} \sim c_{1,\gamma}$ and $\xi L_{2,\gamma} \sim c_{2, \gamma}$, with $c_{1,\gamma},c_{2,\gamma}$ defined in \eqref{eq:L1g-spec-to-time} and \eqref{eq:L2g-spec-to-time} respectively. This shows that, under condition \eqref{prop:item-spec-to-time-bound-1}, $X_n$ satisfies Definition \ref{defn:clm-time-bound} with the constants specified in \eqref{eq:phi-cgamma-boun-spec-to-time}--\eqref{eq:L2g-spec-to-time}.

Let, now, $d_- = 0$ and $L_f^-(x) \sim c \in [0,\infty)$ as $x \to \infty$. Then,
\begin{equation}
\begin{split}
    \int_0^{\lambda_0} \cos(h \om ) L_{f}^- \left(\frac{1}{\om}\right) d\om = \frac{1}{h} \left( \int_0^{\lambda_0} h \cos(h \om ) c d\om  + \int_{ 1/ \lambda_0}^\infty \frac{h\cos(h/\om)}{\om^2} (L_f^- \left(  \om  \right) - c) d\om   \right),
\end{split}
\end{equation}
where the first equality follows from the change of variables $x \mapsto \frac{1}{\om}$ and similarly,
\begin{equation}
 \int_0^{\lambda_0} \sin(h \om ) L_{f}^-\left(\frac{1}{\om}\right) d\om = \frac{1}{h} \left( \int_0^{\lambda_0} h \sin (h \om ) c d\om  + \int_{ 1/ \lambda_0}^\infty \frac{h\sin(h/\om)}{\om^2} (L_f^- \left(  \om  \right) - c) d\om   \right).
\end{equation}
Now note that, 
\[
 \int_0^{\lambda_0} h \cos(h \om ) c d\om = c \sin(h \lambda_0) = O(1), \quad \int_0^{\lambda_0} h \sin (h \om ) c d\om = O(1)
\]
and moreover, for all $\kappa \ge \frac{1}{\lambda_0}$
\[
 \int_{ 1/ \lambda_0}^\kappa \frac{h\cos(h/\om)}{\om^2}  d\om = \sin(h/ \kappa) - \sin(h \lambda_0) \le 2.
\]
In this last display, note that the bound does not depend on $h$. Moreoverer, $L_f^-(x) - c \to 0$ and is non-increasing, and so from Dirichlet's test for the convergence of improper integrals, we deduce that
\[
\int_{ 1/ \lambda_0}^\infty \frac{h\cos(h/\om)}{\om^2} (L_f^- \left(  \om  \right) - c) d\om, \int_{ 1/ \lambda_0}^\infty \frac{h\sin(h/\om)}{\om^2} (L_f^- \left(  \om  \right) - c) d\om 
\]
exist and are upper bounded by a constant that does not depend on $h$ (since the bound above does not depend on $h$). Therefore
\[
\int_0^{\lambda_0} \cos(h \om ) L_{f}^- \left(\frac{1}{\om}\right) d\om = h^{-1} O(1), \quad \int_0^{\lambda_0} \sin(h \om ) L_{f}^-\left(\frac{1}{\om}\right) d\om = h^{-1} O(1),
\]
and so
\begin{equation} \label{eq:border-g-2}
\gamma_-(h) = \cos(\lambda_0 h) h^{-1} O(1) + \sin(\lambda_0 h) h^{-1} O(1).
\end{equation}
Combining \eqref{eq:bound-g+} with \eqref{eq:border-g-2}, we have that
\begin{equation} \label{eq:border-gamma-x}
\begin{split}
    \gamma_X(h) &= 2 \gamma_{+}(h) + 2 \gamma_-(h) \\
    &= c_\gamma \cos(\lambda_0 h + \phi) h^{2d_+-1} \\
    &\quad+ 2 \Gamma(1-2d_+ + \veps) \sin((d_+ - \veps/2) \pi) \tilde L_{f}^+\left(h \right) \cos(\lambda_0 h) h^{2d_+-1 - \veps} \\
   &\quad-  2 \Gamma(1-2d_+ + \veps) \cos((d_+ - \veps/2) \pi) \tilde L_{f}^+\left(h \right) \sin(\lambda_0 h) h^{2d_+-1 - \veps} \\
    &\quad   + o(h^{2d_+-1 - \veps}) + (\cos(\lambda_0 h) + \sin(\lambda_0 h) )h^{-1} O(1) \\
    &=   c_\gamma \cos(\lambda_0 h + \phi) h^{2d-1} + L_{1,\gamma}(h) \cos(\lambda_0 h) h^{2\delta -1}   +  L_{2,\gamma}(h) \sin(\lambda_0 h)) h^{2\delta -1},
\end{split}
\end{equation}
where $\delta = d_+ - \veps / 2$, $L_{1,\gamma}(x) \sim c_{1,\gamma}$ and $\xi L_{2,\gamma}(x) \sim c_{2, \gamma}$, with $c_{1,\gamma},c_{2,\gamma}$ defined in \eqref{eq:L1g-spec-to-time} and \eqref{eq:L2g-spec-to-time} respectively. This shows that, under condition \eqref{prop:item-spec-to-time-bound-2}, $X_n$ satisfies Definition \ref{defn:clm-time-bound} with the constants specified in \eqref{eq:phi-cgamma-boun-spec-to-time}--\eqref{eq:L2g-spec-to-time}.

Finally, let $d_- = 0$ and $L_f^-(x)$ be a differentiable function in $x$ with a bounded derivative. Then, it is immediate that
\begin{equation}
    \int_0^{\lambda_0} \cos(h \om ) L_{f}^- \left(\frac{1}{\om}\right) d\om = \frac{1}{h} \left( L_f^-\left(\frac{1}{\lambda_0}\right) \sin(h\lambda_0) - \int_0^{\lambda_0} \sin(h \om) (L_{f}^-)' \left(\frac{1}{\om}\right) d\om   \right) = h^{-1} O(1),
\end{equation}
where the last inequality follows upon noticing that $(L_{f}^-)'$ is bounded and similarly, 
\begin{equation}
    \int_0^{\lambda_0} \sin(h \om ) L_{f}^- \left(\frac{1}{\om}\right) d\om = h^{-1} O(1).
\end{equation}
Combining the two displays above, we have that $\gamma_-(h) = \cos(\lambda_0 h) h^{-1} O(1) + \sin(\lambda_0 h) h^{-1} O(1) $, which, together with \eqref{eq:bound-g+}, yields the same calculations as in \eqref{eq:border-gamma-x}. This shows that under condition \eqref{prop:item-spec-to-time-bound-3}, $X_n$ again satisfies Definition \ref{defn:clm-time-bound} with the constants specified in \eqref{eq:phi-cgamma-boun-spec-to-time}--\eqref{eq:L2g-spec-to-time}.
\end{proof}

\begin{remark}
    Note that, if conditions \eqref{prop:item-spec-to-time-bound-2} or \eqref{prop:item-spec-to-time-bound-3} are true in Proposition \ref{it:spec-to-time-border}, then $\veps < 2(d_+ - d_-) = 2d_+$, and so $c_{1,\gamma},c_{2,\gamma}$ are given by the third case in \eqref{eq:L1g-spec-to-time} and \eqref{eq:L2g-spec-to-time}.
\end{remark}

\section{Auxiliary Lemmas} \label{app:sec-auxillary}

We present here results on higher-order behavior of the Fourier series (integrals, resp.) of power-law coefficients (functions, resp.) that were used in Appendix \ref{App:subsec-boundary}.

\begin{lemma} \label{lemma:second-order-time-to-spec}
   For $d \in (0,1/2)$, as $\om \to 0^+$,
    \begin{equation}
    \begin{split}
       \sum_{k=1}^\infty \sin(k \om) k^{2d-1} = \om^{-2d} \Gamma(2d) \sin(\pi d) + R_1(\om), \\
       \sum_{k=1}^\infty \cos(k \om) k^{2d-1} = \om^{-2d} \Gamma(2d) \cos(\pi d) + R_2(\om),
    \end{split}
    \end{equation}
    where $R_i(\om) \to c_i \in \RR$, $i=1,2$.
    % or with $p=1-2d \in (0,1)$
    % \[
    % \sum_{k=1}^\infty \sin(k \om) k^{-p} = \om^{p-1} \Gamma(1-p) \cos\left( p \frac{\pi}{2}\right) + R(\om),
    % \]
    % where the remainder term $R(\om) \to C \in \RR$ as $\om \to 0^+$. 
\end{lemma}

\begin{proof}
    Write
    \begin{equation} \label{eq:lemma-aux-1}
    \begin{split}
        \int_0^\infty e^{iu \om} u^{2d-1} du - \sum_{k=1}^\infty e^{ik\om} k^{2d-1} &= \sum_{k=1}^\infty \left( \int_{k-1}^{k} e^{iu \om} u^{2d-1} du -  e^{ik\om} k^{2d-1}  \right) \\
        &=\sum_{k=1}^\infty \left( \int_{k-1}^{k} e^{iu\om} (u^{2d-1} - k^{2d-1})du  + k^{2d-1}  \left( \int_{k-1}^{k} e^{iu\om} du - e^{ik\om}  \right)   \right) .
    \end{split}
    \end{equation}
    Next, note that
    \begin{equation}
        \int_{k-1}^{k} (u^{2d-1} - k^{2d-1}) du = k^{2d} \int_{1-1/k}^{1} (z^{2d-1} -1) dz =  -k^{2d-2} \frac{2d-1}{2},
    \end{equation}
    which implies,
    % \begin{equation} 
    %     \left| \sum_{k=1}^\infty \int_k^{k+1} e^{iu \om} (u^{2d-1} - k^{2d-1}) du  \right| \le \sum_{k=1}^\infty \int_k^{k+1}  (k^{2d-1} - u^{2d-1}) du = C \in \RR_+,
    % \end{equation}
    % and so, 
    from the bounded convergence theorem, as $\om \to 0^+$,
    \begin{equation} \label{eq:lemma-aux-2}
        \sum_{k=1}^\infty \int_{k-1}^{k} e^{iu \om} (u^{2d-1} - k^{2d-1}) du \to - C.
    \end{equation}
    Moreover, a simple estimate shows that
    \begin{equation}
        \int_{k-1}^{k} e^{iu\om} du - e^{ik\om} = \frac{e^{i\om k } - e^{i\om (k-1)}}{i\om} - e^{i\om k} = e^{i k \om} \frac{1 - e^{- i \om}   -i \om}{i \om}.
    \end{equation}
    Thus,
    \begin{equation} \label{eq:lemma-aux-3}
        \sum_{k=1}^\infty k^{2d-1}  \left( \int_k^{k+1} e^{iu\om} du - e^{ik\om}  \right) = \frac{1 - e^{- i \om}   -i \om}{i \om} \sum_{k=1}^\infty (k^{2d-1} e^{ik \om}) \sim  \om^{-2d+1} \Gamma(2d) e^{i \pi (\frac{1}{2} - d) } = o(1),
    \end{equation}
    where the last asymptotic relation holds from Proposition A.2.1 of \cite{pipiras_taqqu_2017}. 
    By combining \eqref{eq:lemma-aux-1}, \eqref{eq:lemma-aux-2}, and \eqref{eq:lemma-aux-3},
    \begin{equation}
    \begin{split}
        \sum_{k=1}^\infty e^{ik\om} k^{2d-1} &=  \int_0^\infty e^{iu \om} u^{2d-1} du  \\
        &\quad-\sum_{k=1}^\infty  \int_{k-1}^{k} e^{iu\om} (u^{2d-1} - k^{2d-1})du  - \sum_{k=1}^\infty k^{2d-1}  \left( \int_{k-1}^{k} e^{iu\om} du - e^{ik\om}  \right)   \\
        &= \om^{-2d} \Gamma(2d) e^{i d \pi}  + R(\om),
    \end{split}
    \end{equation}
    where, as $\om \to 0^+$, $R(\om) \to C - \frac{1}{2d}$ and $C$ is given in \eqref{eq:lemma-aux-2}.
\end{proof}

\begin{lemma} \label{lemma-second-order-spec-to-time}
    Let $ d \in \left(0, \frac{1}{2} \right)$. Then, as $h \to \infty$,
    \begin{equation}
    \begin{split}
            \int_0^{1}  \cos(h  \om )  \om^{-2d} d\om &= \Gamma(1-2d) \sin(\pi d) h^{2d-1} + \sin(h) h^{-1} + O(h^{-2}), \\
            \int_0^{1} \sin(h  \om )  \om^{-2d} d\om &= \Gamma(1-2d) \cos(\pi d) h^{2d-1} - \cos(h) h^{-1} + O(h^{-2}).
    \end{split}
    \end{equation}
\end{lemma}

\begin{proof}
    We prove the equivalent identity
    \begin{equation}
        \int_0^{1}  e^{i h \om}  \om^{-2d} d\om = \Gamma(1-2d) e^{i \pi (\frac{1}{2} - d) } h^{2d-1} - i e^{ih} h^{-1} + O(h^{-2}).
    \end{equation}
    Write 
    \begin{equation} \label{eq-fourier-power-law-1}
        \int_0^{1}  e^{i h \om}  \om^{-2d} d\om = \int_0^\infty  e^{i h \om}  \om^{-2d} d\om - \int_{1}^\infty  e^{i h \om}  \om^{-2d} d\om,
    \end{equation}
    where
    \begin{equation} \label{eq-fourier-power-law-2}
        \int_0^\infty  e^{i h \om}  \om^{-2d} d\om = h^{2d-1} \int_0^\infty e^{iz} z^{-2d} dz = \Gamma(1-2d) e^{i \pi (\frac{1}{2} - d) } h^{2d-1}.
    \end{equation}
    Moreover, 
    \begin{equation} \label{eq-fourier-power-law-3}
    \begin{split}
      \int_{1}^\infty  e^{i h \om}  \om^{-2d} d\om &= h^{2d-1} \int_h^\infty e^{iz} z^{-2d} dz \\
      &= h^{2d-1}  \int_{h}^\infty  e^{i z}  z^{-2d} dz \\
      &= h^{2d-1} \left( h^{-2d} e^{iz} i - 2d h^{-2d-1} e^{ih} + O(h^{-2d-3} )   \right) \\
      &= e^{iz} i h^{-1} + O(h^{-2}).
    \end{split}
    \end{equation}
    Combining \eqref{eq-fourier-power-law-1}, \eqref{eq-fourier-power-law-2}, and \eqref{eq-fourier-power-law-3} we obtain the desired result.
\end{proof}
