# Supplementary material for: Cyclical Long Memory: Decoupling, Modulation, and Modeling
Source: arXiv:2403.07170 source file (2024-07-04)
Supplement: Supplementary file 2 [file Old_thoughts_-_appendix.tex]

\section{Definitions of CLM} \label{appendix:acvf-spec-clm}
\normalsize

We first recall two definitions related to slowly varying functions. These conditions will be useful in the formulation of the results below.

A slowly varying function $L$ is called \textit{quasi-monotone} (see, e.g., Chapter 2.7 in \cite{bingham_goldie_teugels_1987}) if the following two conditions hold: $(i)$ it is of bounded variation on any compact interval of $[0,\infty)$ and $(ii)$ for some $\delta > 0$,
\[
\int_0^x u^\delta |d L(u)| = O(x^\delta L(x)), \quad \text{as } x \to \infty.
\]
A measurable function $f$ \textit{belongs to the Zygmund class} if, for every $\alpha > 0$, $x^\alpha f(x)$ is ultimately increasing and $x^{-\alpha} f(x)$ is ultimately decreasing, i.e., there exists some $M \in \RR_+$ such that $x^{\alpha} f(x)$ is increasing in $[M,\infty)$ (resp. $x^{-\alpha} f(x)$ is decreasing in $[M,\infty)$). The Zygmund class coincides with that of the normalized slowly varying functions, see, e.g., Chapter 1.5.3 of \cite{bingham_goldie_teugels_1987}.

We now present the formal definitions for (symmetric) CLM.

\begin{defn}(Time domain) \label{defn:clm-time}
    A second-order stationary time series $\{X_n\}_{n \in \ZZ}$ is said to exhibit CLM if its autocovariance function satisfies
    \begin{equation} \label{eq:def-eq-acvf}
        \gamma_X(h) = L_{1,\gamma}(h) \cos(\lambda_0 h) h^{2d-1} + L_{2,\gamma}(h) \sin(\lambda_0 h) h^{2d-1} , \quad h \in \ZZ,
    \end{equation}
    where $L_{1,\gamma}, L_{2,\gamma} : \ZZ \to \RR$ are symmetric functions around $0$ with $L_{1,\gamma}(h) \sim c_{1,\gamma} \in (0,\infty)$ and $L_{2,\gamma}(h) \sim c_{2,\gamma} \in (0,\infty)$ as $h \to \infty$, $\lambda_0 \in (0,\pi)$, and $d \in (0,1/2)$ is the memory parameter. 
\end{defn}

\begin{remark} \label{rmk-clm-defn-time-equiv}
    Note that \eqref{eq:def-eq-acvf} in Definition \ref{defn:clm-time} can be recast as
    \begin{equation}
    \gamma_X(h) = c_\gamma \cos(\lambda_0 h + \phi)  h^{2d-1} + R(h),
    \end{equation}
    where
    \begin{equation} \label{eq:rig-c1g-c2g-c-psi}
         c_\gamma \doteq \sqrt{(c_{1,\gamma})^2 + (c_{2,\gamma})^2}, \quad \phi \doteq \arcsin\left(  \frac{- c_{2,\gamma}}{\sqrt{(c_{1,\gamma})^2 + (c_{2,\gamma})^2}}\right),
    \end{equation}
    and 
    \[
    R(h) \doteq (L_{1,\gamma}(h) - c_{1,\gamma}) \cos(\lambda_0 h ) h^{2d-1} + (L_{2,\gamma}(h) - c_{2,\gamma}) \sin(\lambda_0 h ) h^{2d-1} = o(h^{2d-1}),
    \]
    since $L_{1,\gamma}(h) \sim c_{1,\gamma}$ and $L_{2,\gamma}(h) \sim c_{2,\gamma}$ as $h \to \infty$. 
\end{remark}

\begin{defn}(Spectral domain) \label{defn:clm-spec}
    A second-order stationary time series $\{X_n\}_{n \in \ZZ}$ is said to exhibit CLM if its spectral density satisfies
\begin{equation} \label{eq:spec-rigorous-defn}
    f_X(\lambda) = \begin{cases}
        L_f^- \left(\frac{1}{\lambda_0 - \lambda}\right)  (\lambda_0 - \lambda)^{-2d}, & 0 < \lambda < \lambda_0, \vspace{3mm}\\
        L_f^+ \left(\frac{1}{\lambda - \lambda_0}\right)  (\lambda - \lambda_0)^{-2d}, & \lambda_0 < \lambda < \pi,
    \end{cases}
\end{equation}
where $L_f^-: \left(\frac{1}{\lambda_0},\infty\right) \to (0,\infty)$ and $L_f^+: \left(\frac{1}{\pi - \lambda_0},\infty\right) \to (0,\infty)$ are two functions such that $L_f^+ \sim c_f^+$ and $L_f^- \sim c_f^-$ as $h \to + \infty$, where $c_f^\pm \in (0,\infty)$.
\end{defn}

Definitions \ref{defn:clm-time} and \ref{defn:clm-spec} are, in general, not equivalent. We are ready to formulate the result that establishes the connection between these two definitions.
\begin{proposition} \label{prop:equiv-defn}
\begin{enumerate}[(i)]
    \item Suppose that $L_{1,\gamma}, L_{2,\gamma}$ are slowly varying functions at $+ \infty$ that belong to the Zygmund class. Then, Definition \ref{defn:clm-time} implies Definition \ref{defn:clm-spec} with 
    \begin{equation}
        c_f^\pm \doteq \frac{\Gamma(2d)}{2\pi} \left( c_{1,\gamma} \cos(d \pi) \mp c_{2,\gamma} \sin(d \pi) \right).
    \end{equation}
    \item Suppose that $L_f^+,L_f^-$ are quasi-monotone slowly varying functions at $+ \infty$. Then, Definition \ref{defn:clm-spec} implies Definition \ref{defn:clm-time} (uner the formulation of Remark \ref{rmk-clm-defn-time-equiv}) with
    \begin{equation} \label{eq:cgamma-psi}
   \begin{split}
    &c_\gamma \doteq 2\Gamma(1-2d) \sqrt{(c_f^+ + c_f^-)^2 \sin(\pi d)^2 + (c_f^+ - c_f^-)^2 \cos^2(\pi d)} \\
    &\quad= 2\Gamma(1-2d)\sqrt{(c_f^+)^2 + (c_f^-)^2 - 2 c_f^+ c_f^-\cos^2(2 \pi d)} \\
    &\phi \doteq  \arcsin \left( \frac{(c_f^+ - c_f^-) \cos(\pi d)}{\sqrt{(c_f^+)^2 + (c_f^-)^2 - 2 c_f^+ c_f^-\cos^2(2 \pi d)}}  \right).
   \end{split}
\end{equation}
\end{enumerate}
\end{proposition}

We start by presenting a Lemma addressing the second order behavior of the Fourier series of power-law coefficients.

\begin{lemma}
    For $d \in (0,1/2)$, as $\om \to 0^+$,
    \[
    \sum_{k=1}^\infty \cos(k \om) k^{2d-1} = \om^{-2d} \Gamma(2d) \cos(\pi d) + O(1),
    \]
    or with $p=1-2d \in (0,1)$
    \[
    \sum_{k=1}^\infty \cos(k \om) k^{-p} = \om^{p-1} \Gamma(1-p) \sin\left( p \frac{\pi}{2}\right) + O(1).
    \]
\end{lemma}

\begin{proof}
    Define, for fixed $p \in (0,1)$, $g(x) \doteq x^{2-p}$. Then, $g$ is clearly twice differentiable and it admits the following expansion
    \[
    \frac{\left(  1 + \frac{1}{k} \right)^{2-p} - 2 + \left(  1 - \frac{1}{k} \right)^{2-p}}{\frac{1}{k^2}} = g''(1) + O\left(\frac{1}{k^2}\right)
    \]
    or, since $g(1) = 1, g''(1) = (2-p)(1-p)$, 
    \begin{equation} \label{eq:power-law-1}
        k^{-p} = \frac{(k+1)^{2-p} - 2k^{2-p} + (k-1)^{2-p}}{(2-p)(1-p)}  + O\left(\frac{1}{k^{2+p}}\right).
    \end{equation}
    Then, by using \eqref{eq:power-law-1},
    \begin{equation}
        \sum_{k=1}^\infty \cos(k\om) k^{-p} = \sum_{k=1}^\infty \cos(k\om) \frac{(k+1)^{2-p} - 2k^{2-p} + (k-1)^{2-p}}{(2-p)(1-p)} + \sum_{k=1}^\infty \cos(k \om) O\left(\frac{1}{k^{2+p}}\right),
    \end{equation}
    where, since $2+p > 1$,
    \[
    \sum_{k=1}^\infty \cos(k \om) O\left(\frac{1}{k^{2+p}}\right) = O(1).
    \]
    This implies that
    \begin{equation}
        \sum_{k=1}^\infty \cos(k\om) k^{-p} 
        = \frac{2\pi}{(2-p)(1-p)} f_Z(\om)  + O(1)
    \end{equation}
    where $Z$ is a standard fractional Gaussian noise with Hurst parameter $H=1 - \frac{p}{2}$ and spectral density 
    \[
    f_Z(\om) = \left[ \frac{1}{2\pi} \sum_{k=-\infty}^\infty e^{-ik\om}  \frac{|k+1|^{2-p} - 2 |k|^{2-p} + |k-1|^{2-p}}{2}   \right].
    \]
    Let, as in Proposition 2.6.11 of \cite{pipiras_taqqu_2017},
    \[
    \left(c_2\left(1- \frac{p}{2}\right)\right)^2 \doteq \int_\RR |e^{ix} -1 |^2 |x|^{-p-3} \hat{B}(dx) = \frac{2\pi}{(2-p)(1-p)\Gamma(2-p) \sin\left(\frac{p}{2} \pi \right)}, 
    \]
    where $\hat B(dx)$ is a Hermitian Gaussian random measure with control measure $\EE |\hat{B}(dx) |^2 = dx$ and the second equality follows from display (2.6.10) of \cite{pipiras_taqqu_2017}. Then,
    \begin{equation}
    \begin{split}
        \sum_{k=1}^\infty \cos(k\om) k^{-p} &= \frac{2\pi}{(2-p)(1-p)} \frac{1}{c_2\left(1-\frac{p}{2}\right)^2} |1-e^{-i\om}|^2 \sum_{n=-\infty}^\infty |\om + 2\pi n|^{-1-2+p} \\
        &= \Gamma(1-p) \sin \left( \frac{p}{2} \pi  \right) |1-e^{-i\om}|^2 |\om|^{p-3} + O(1)
    \end{split}
    \end{equation}
    \PZ{this $\om$ comes from where?}where the first line follows from Proposition 2.8.1 of \cite{pipiras_taqqu_2017}. Finally, remark that
    \[
    |1-e^{-i\om}|^2 = (1-\cos(\om))^2 + \sin^2(\om) = 4 \sin^2 \left( \frac{\om}{2} \right) = \om^2 + O(|\om|^6),
    \]
    which says that
    \[
    \sum_{k=1}^\infty \cos(k\om) k^{-p} = \Gamma(1-p) \sin \left( \frac{p}{2} \pi  \right) |\om|^{p-1} + O(1).
    \]
    This proves the desired equality.
\end{proof}

\subsection{From spectral to time domain (proof of Prop. \ref{prop:equiv-defn}(ii))} \label{app:subsec:spec-to-time}

\begin{proof}
Let the spectral density $f_X$ of $X$ be given by \eqref{eq:spec-rigorous-defn}. Then, 
\begin{equation} \label{eq:210}
\begin{split}
\gamma_X(h) &=   2\int_{0}^{\pi} \cos(h\lambda) f_X(\lambda) d\lambda  = 2 \int_0^{\lambda_0} \cos(h\lambda) f_X(\lambda) d\lambda + 2 \int_{\lambda_0}^{\pi} \cos(h\lambda) f_X(\lambda) d\lambda \\
&\doteq 2\left[ \gamma_-(h) + \gamma_+(h)   \right].
\end{split}
\end{equation}
We compute these two quantities separately. First,
\begin{equation}
\begin{split}
    \gamma_-(h) &= \int_0^{\lambda_0} \cos(h \lambda ) L_f^-\left( \frac{1}{\lambda_0 - \lambda}\right) (\lambda_0 - \lambda)^{-2d}   d\lambda \\
    &= \int_0^{\lambda_0} \cos(h (\lambda_0 - \om)) L_f^-\left( \frac{1}{\om} \right) \om^{-2d}   d\om \\
    &= \cos(h \lambda_0) \int_0^{\lambda_0} \cos(h \om)  L_f^-\left( \frac{1}{\om} \right) \om^{-2d}   d\om + \sin(h \lambda_0) \int_0^{\lambda_0} \sin(h \om)  L_f^-\left( \frac{1}{\om} \right) \om^{-2d}   d\om
\end{split}
\end{equation}
where the second line follows from the change of variables $\lambda_0 - \lambda \to \om$. By Proposition A.2.2 of \cite{pipiras_taqqu_2017} and since $L_f^-$ is quasi-monotone, we have that
\begin{equation}
    \int_0^{\lambda_0} \cos(h \om)  L_f^-\left( \frac{1}{\om} \right) \om^{-2d}   d\om \sim h^{2d-1} L_f^-(h) \Gamma(1-2d) \sin(\pi d),
\end{equation}
and similarly
\begin{equation}
    \int_0^{\lambda_0} \sin(h \om)  L_f^-\left( \frac{1}{\om} \right) \om^{-2d}   d\om  \sim h^{2d-1} L_f^-(h) \Gamma(1-2d) \cos(\pi d).
\end{equation}
Analogous calculations show that,
\begin{equation}
\begin{split}
    \gamma_+(h) &= \int_{\lambda_0}^\pi \cos(h \lambda ) L_f^+\left( \frac{1}{\lambda_0 - \lambda}\right) (\lambda_0 - \lambda)^{-2d}   d\lambda \\
    &= \int_0^{\pi - \lambda_0} \cos(h (\lambda_0 + \om)) L_f^+\left( \frac{1}{\om} \right) \om^{-2d}   d\om \\
    &= \cos(h \lambda_0) \int_0^{\pi - \lambda_0} \cos(h \om)  L_f^+\left( \frac{1}{\om} \right) \om^{-2d}   d\om - \sin(h \lambda_0) \int_0^{\pi - \lambda_0} \sin(h \om)  L_f^+\left( \frac{1}{\om} \right) \om^{-2d}   d\om,
\end{split}
\end{equation}
where
\begin{equation}
    \int_0^{\pi - \lambda_0} \cos(h \om)  L_f^+\left( \frac{1}{\om} \right) \om^{-2d}   d\om \sim h^{2d-1} L_f^+(h) \Gamma(1-2d) \sin\left( \pi d   \right),
\end{equation}
and
\begin{equation}
    \int_0^{\pi - \lambda_0} \sin(h \om)  L_f^+\left( \frac{1}{\om} \right) \om^{-2d}   d\om  \sim h^{2d-1} L_f^+(h) \Gamma(1-2d) \cos\left( \pi d   \right).
\end{equation}
Since $L_f^{\pm}(h) \to c_f^{\pm}$ as $h \to \infty$, by plugging the previous six displays in \eqref{eq:210}, we have that
\begin{equation}
\begin{split}
    \gamma_X(h) &= \cos(h \lambda_0) \left[ h^{2d-1} c_f^- 2 \Gamma(1-2d) \sin(\pi d)  +R_1^-(h)) \right] \\
    &\quad+ \sin(h \lambda_0) \left[ h^{2d-1} c_f^- 2 \Gamma(1-2d) \cos(\pi d)  + R_2^-(h)) \right] \\
    &\quad + \cos(h \lambda_0) \left[ h^{2d-1} c_f^+ 2 \Gamma(1-2d) \sin(\pi d)  + R_1^+(h)) \right] \\
    &\quad- \sin(h \lambda_0) \left[ h^{2d-1} c_f^+ 2 \Gamma(1-2d) \cos(\pi d)  + R_2^+(h)) \right],
\end{split}
\end{equation}
where we have defined $R_{1}^\pm(h) \doteq 2(L_f^\pm(h) - c_f^{\pm}) \Gamma(1-2d) \sin(\pi d) h^{2d-1}$ and $R_{2}^\pm(h) \doteq 2(L_f^\pm(h) - c_f^{\pm}) \Gamma(1-2d) \cos(\pi d) h^{2d-1}$. This says that, by defining $\psi$ and $c_\gamma$ as in \eqref{eq:cgamma-psi}, we have that
\begin{equation} \label{eq:213}
\begin{split}
    \gamma_X(h) &= 2 \Gamma(1-2d) h^{2d-1}  \left[(c_f^+ + c_f^-)  \sin(\pi d) \cos(\lambda_0 h) + (c_f^- - c_f^+)  \cos(\pi d) \sin(\lambda_0h)\right] + R(h) \\
    &= c_\gamma \cos(\lambda_0 h + \phi) h^{2d-1} + R(h),
\end{split}
\end{equation}
where 
\[
R(h) \doteq \cos(h \lambda_0) R_1^-(h) + \sin(h \lambda_0) R_2^-(h) + \cos(h \lambda_0) R_1^+(h) - \sin(h \lambda_0) R_2^+(h).
\]
The result follows upon noticing that $R(h)$ is $o(h^{2d-1})$.
\end{proof}

\begin{remark}
    In particular, when $c_f^+ = c_f^- = c_f$, we get that
\begin{equation} \label{eq:cf-cf+cf}
    c_\gamma = 4 \Gamma(1-2d) c_f \sin(\pi d), \quad \phi = 0.
\end{equation}
% When, e.g., $c_f^+ > 0$ and $c_f^- = 0$, we get that
% \begin{equation} \label{eq:cf-0}
%     c_\gamma = 2 \Gamma(1-2d) c_f^+, \quad \phi =  \left( \frac{1}{2} - d \right) \pi.
% \end{equation}
% When $c_f^- > 0$ and $c_f^+ = 0$, we get that
% \begin{equation} \label{eq:cf+0}
%     c_\gamma = 2 \Gamma(1-2d) c_f^-, \quad \phi = - \left( \frac{1}{2} - d \right) \pi.
% \end{equation}
\end{remark}


\subsection{From time to spectral domain (proof of Prop. \ref{prop:equiv-defn}(i))} \label{app:subsec:time-to-spec}

\begin{proof}
Let the ACVF of $X$ be of the form \eqref{defn:clm-time}, where $L_{1,\gamma}, L_{2,\gamma}$ are slowly varying functions that belong to the Zygmund class. \PZ{First I need to argue that the following representation holds
\begin{equation}
f_X(\lambda) =  \frac{1}{2\pi} \sum_{h=-\infty}^{\infty} e^{-ih\lambda} \gamma_X(h),
\end{equation}
see Proof of Prop. 2.2.14 in the Appendix of \cite{pipiras_taqqu_2017}. TO DO.
}

Then,
\begin{equation} \label{eq:456}
\begin{split}
        f_X(\lambda) &=  \frac{1}{2\pi} \left[ \gamma_X(0) + 2\sum_{h=1}^\infty \cos( h \lambda ) \left(L_{1,\gamma}(h) \cos( \lambda_0 h ) + L_{1,\gamma}(h) \sin( \lambda_0 h ) \right) h^{2d-1} \right] \\ 
    &= \frac{1}{2\pi} \left[ \gamma_X(0) + f_1(\lambda) -  f_2(\lambda) +  f_3(\lambda) + f_4(\lambda) \right] 
\end{split}
\end{equation}
where
\begin{equation}
    f_1(\lambda) \doteq \sum_{h=1}^\infty \cos\big((\lambda-\lambda_0) h \big) L_{1,\gamma}(h) h^{2d-1}, \quad f_2(\lambda) \doteq \sum_{h=1}^\infty \sin\big((\lambda-\lambda_0) h \big) L_{2,\gamma(h)} h^{2d-1}
\end{equation}
and
\begin{equation}
    f_3(\lambda) \doteq  \sum_{h=1}^\infty \cos((\lambda + \lambda_0)h  )  L_{1,\gamma}(h)  h^{2d-1}, \quad f_3(\lambda) \doteq  \sum_{h=1}^\infty \sin((\lambda + \lambda_0)h  )  L_{2,\gamma}(h)  h^{2d-1}.
\end{equation}
By Proposition A.2.1 of \cite{pipiras_taqqu_2017}, as $\lambda \to \lambda_0$, \PZ{Vladas was dividing by $\pi$ but I can't see this in the lemma.}
\begin{equation}
\begin{split}
    f_1(\lambda) &\sim |\lambda-\lambda_0|^{-2d} L_\gamma \left(  \frac{1}{|\lambda - \lambda_0|}  \right) \Gamma(2d) \cos(d\pi), \\
    f_2(\lambda) &\sim \text{sign}(\lambda - \lambda_0) |\lambda-\lambda_0|^{-2d} L_\gamma \left(  \frac{1}{|\lambda - \lambda_0|}  \right) \Gamma(2d) \sin(d\pi).
\end{split}
\end{equation}
On the other hand, by using Lagrange's trigonometric identities, for each $N \in \NN$
\[
\sum_{h=1}^N \cos((\lambda + \lambda_0)h  ) \le \frac{1}{2} + \frac{1}{2 \min\{ \sin\left(\frac{\lambda_0}{2}\right) ,\sin\left(\frac{\pi + \lambda_0}{2}\right)  \}}, \quad \sum_{h=1}^N \sin((\lambda + \lambda_0)h  ) \le \frac{1}{\min\{ \sin\left(\frac{\lambda_0}{2}\right) ,\sin\left(\frac{\pi + \lambda_0}{2}\right)  \}}.
\]
Note that these bounds are uniform in $\lambda$ and that $L_{1,\gamma(h)} h^{2d-1}, L_{2,\gamma(h)} h^{2d-1}$ are eventually decreasing (since $L_{1,\gamma}$ and $L_{2,\gamma}$ belong to the Zygmund class). Therefore, by Dirichlet's test, $f_3(\lambda) \le M, f_4(\lambda) \le M$, for some constant $M$ that does not depend on $\lambda$. By the dominated convergence theorem, there exist constants $\sigma,\tau \in \RR$ with
\[
f_3(\lambda) \sim \sigma < \infty, \quad f_4(\lambda) \sim \tau < \infty,\quad  \text{as } \lambda \to \lambda_0.
\]
Since $L_{1,\gamma(h)} \to c_{1,\gamma}, L_{2,\gamma(h)} \to c_{2,\gamma}$ as $h \to \infty$, we then get, from \eqref{eq:456},
\begin{equation}
    f_X(\lambda) \sim \frac{\Gamma(2d)}{2\pi} \left[ c_{1,\gamma} \cos(d\pi) - \text{sign}(\lambda-\lambda_0) c_{2,\gamma} \sin(d\pi)   \right]    | \lambda - \lambda_0 |^{-2d}.
\end{equation}
This concludes the result.
\end{proof}

\begin{remark}
    From the calculations above, we obtain the following relationship relating  $c_f^+,c_f^-$ with $c_\gamma,\phi$ defined in \eqref{rmk-clm-defn-time-equiv}:
        \begin{equation} \label{eq:cfpm-cgamma}
    c_f^\pm = \frac{c_\gamma}{2\pi} \Gamma(2d) \cos(d\pi \mp \phi).
\end{equation}
Indeed, this follows by writing
\begin{equation}
\begin{split}
    f_X(\lambda) &\sim \frac{\Gamma(2d)}{2\pi} \left[ c_{1,\gamma} \cos(d\pi) - \text{sign}(\lambda-\lambda_0) c_{2,\gamma} \sin(d\pi)   \right]    | \lambda - \lambda_0 |^{-2d} \\
    &= \frac{\Gamma(2d)}{2\pi} c_\gamma \left[ \cos(\phi) \cos(d\pi) + \text{sign}(\lambda-\lambda_0) \sin(\phi) \sin(d\pi) \right] | \lambda - \lambda_0 |^{-2d} \\
    &=  \frac{\Gamma(2d)}{2\pi} c_\gamma \cos(d\pi - \text{sign}(\lambda-\lambda_0)\phi)  | \lambda - \lambda_0 |^{-2d}.
\end{split}
\end{equation}
\end{remark}

\subsection{Set of admissible cyclical phases}
\label{subsubsec:admis-phase}

Since $c_f^+,c_f^- \ge 0$, note that \eqref{eq:cfpm-cgamma} yields
\[
-\frac{\pi}{2} < d\pi - \phi < \frac{\pi}{2}, -\frac{\pi}{2} <  \phi - d\pi < \frac{\pi}{2}
\]
so that, as stated in \eqref{eq:admiss-sets-def},
\[
\phi \in \cli_d = \left[\left(d - \frac{1}{2} \right)\pi  , \left(\frac{1}{2} - d\right) \pi \right].
\]
% As in \eqref{eq:cf-0} and \eqref{eq:cf+0}, note again that the boundary values $\phi = \pm \left(\frac{1}{2}-d\right) \pi$ correspond to $c_f^\mp = 0$.

\subsection{Boundary case}

As anticipated, the boundary cases $\phi = \pm \left(d - \frac{1}{2} \right) \pi$ need special treatment. Without loss of generality, suppose that $\phi =  \left(d - \frac{1}{2} \right) \pi$. We

\textbf{time to spectral domain}
Let $\delta < d$, and define $\psi \doteq  \pm \left( \frac{1}{2} - d\right) \pi $. Then
\[
\gamma_X(h) = c_\gamma \cos(\lambda_0 h + \psi) h^{2d-1} + L_{1,\gamma}(h) \cos(\lambda_0 h) h^{2\delta-1} + L_{2,\gamma}(h) \sin(\lambda_0 h) h^{2\delta-1} = \gamma_1(h) + \gamma_2(h),
\]
with
\[
\gamma_1(h) \doteq  c_\gamma \cos(\lambda_0 h + \psi) h^{2\delta-1}, \quad \gamma_2(h) \doteq L_{1,\gamma}(h) \cos(\lambda_0 h) h^{2\delta-1} + L_{2,\gamma}(h) \sin(\lambda_0 h) h^{2\delta-1}.
\]

\textbf{First, assume that $0 < \delta < d$}, then from calculations as in ..., 
\[
\sum_{h=-\infty}^\infty e^{-ih\lambda} \gamma_{x,2} (h) \sim \frac{\Gamma(2d)}{2\pi} \left[ c_{1,\gamma} \cos(d\pi) - \text{sign}(\lambda-\lambda_0) c_{2,\gamma} \sin(d\pi)   \right] |\lambda - \lambda_0|^{-2\delta}.
\]
On the other hand, as $\lambda \to \lambda_0^-$,
\begin{equation}
\begin{split}
  \sum_{h=-\infty}^\infty e^{-ih\lambda} \gamma_{X,1}(h) &= \sum_{h=-\infty}^\infty e^{-ih\lambda} c_\gamma \cos(\lambda_0 |h| + \psi) |h|^{2d-1} \\
&= \frac{1}{2\pi} \left[ \gamma_X(0) + \cos(\psi) f_1(\lambda) -  \sin(\psi) f_2(\lambda) +  f_3(\lambda) + f_4(\lambda) \right]  \\
&= \left[ \cos(\psi) \cos(\pi d) + \text{sign}(\lambda - \lambda_0) \sin(\psi) \sin(\pi d) \right]  c_\gamma \frac{1}{2\pi} |\lambda - \lambda_0|^{-2d} + O(1) = O(1),
\end{split}
\end{equation}
which says that, in this case,
\[
f_X(\lambda) \sim \begin{cases}
    \frac{\Gamma(2d)}{2\pi} \left[ c_{1,\gamma} \cos(d\pi) - \text{sign}(\lambda-\lambda_0) c_{2,\gamma} \sin(d\pi)   \right] |\lambda - \lambda_0|^{-2\delta} & \lambda \to \lambda_0^- \\
    \cos(2\pi d) \frac{c_\gamma}{2\pi} |\lambda - \lambda_0|^{-2d} &  \lambda \to \lambda_0^+
\end{cases}
\]

\textbf{Now investigate the case $\delta < 0$}. Here, we have that
\[
| \sum_{h=-\infty}^\infty e^{-ih\lambda} \gamma_{X,1}(h) | \le \sum_{h=-\infty}^\infty O(|h|^{2\delta-1}) = O(1),
\]
which says that, as $h \to \infty$,
\[
\sum_{h=-\infty}^\infty \cos(h\lambda) \gamma_{X,1}(h) + \sum_{h=-\infty}^\infty \cos(h\lambda) \gamma_{X,2}(h) \sim \nu > 0. 
\]
Then,
\[
f_X(\lambda) \sim \begin{cases}
    \nu & \lambda \to \lambda_0^- \\
    \cos(2\pi d) \frac{c_\gamma}{2\pi} |\lambda - \lambda_0|^{-2d} &  \lambda \to \lambda_0^+
\end{cases}
\]

\textbf{Finally, the case $\delta = 0$.\footnote{Note that, in the terminology of \cite{bingham_goldie_teugels_1987}, the results of Zygmund hold for slowly varying functions in the Zygmund class.\cite{bingham_goldie_teugels_1987} presents the result for sines in Section 4.3, but I cannot find the one for cosines there, so I will cite the book of Zygmund instead}} 

This is the most delicate case. We see that, for a slowly varying function $l$ that is in the Zygmund class, as $\lambda \to 0+$
\[
\sum_{h=1}^\infty \frac{\sin{h \lambda}}{h} \sim \frac{\pi}{2}
\]
(Theorem 5.2.6 in Zygmund and the remark that follows the proof with $\beta = 1$). Moreover, as $\lambda \to 0+$
\[
\sum_{h=1}^\infty \frac{\cos{h \lambda}}{h} \sim \log\left( |\lambda^{-1}| \right)
\]
(Theorem 5.2.15 in Zygmund). Alltogether, these say that
\[
f_X(\lambda) \sim \begin{cases}
   | \log \left(|\lambda -\lambda_0|^{-1}\right) | & \lambda \to \lambda_0^- \\
    \cos(2\pi d) \frac{c_\gamma}{2\pi} |\lambda - \lambda_0|^{-2d} &  \lambda \to \lambda_0^+
\end{cases}
\]

\textbf{spectral domain to time domain}.

We now turn to obtaining the asymptotics in the time domain from the spectral domain in the boundary case. 

\begin{proposition}
    \begin{enumerate}[(i)]
        \item If $f_X(\lambda) = L_{f,1}(\lambda) |\lambda - \lambda_0|^{-2\delta} 1_{(0,\lambda_0)}(\lambda) +  L_{f,2}(\lambda) |\lambda - \lambda_0|^{-2d} 1_{(\lambda_0,\pi)}(\lambda) L(|\lambda - \lambda_0|^{-1})$ with $0 < \delta < d$ and where $L_{f,1}$ is a slowly varying function of bounded variation in $(0,\lambda_0 - \varepsilon)$ and $L_{f,2}$ is a slowly varying function of bounded variation in $(\lambda_0 +\varepsilon,\pi)$ for all $\varepsilon>0$.
        
        \item If $f_X(\lambda) = L_{f,1}(\lambda) 1_{(0,\lambda_0)}(\lambda) +  L_{f,2}(\lambda) |\lambda - \lambda_0|^{-2d} 1_{(\lambda_0,\pi)}(\lambda) L(|\lambda - \lambda_0|^{-1})$, where $L_{f,2}$ is as before and $L_{f,1}$ is a slowly varying function of bounded variation in $(0,\lambda_0)$ with $L_{f,1}(\lambda) \to c \neq 0$ as $\lambda \to \lambda_0^-$. Then...
        \[
        \gamma_X(h) =
        \]
        \item If $f_X(\lambda) = |\log((\lambda_0 - \lambda)^{-1})| 1_{(0,\lambda_0)}(\lambda) +  L_{f,2}(\lambda) |\lambda - \lambda_0|^{-2d} 1_{(\lambda_0,\pi)}(\lambda) L(|\lambda - \lambda_0|^{-1})$, where $L_{f,2}$ is as before and $L_{f,1}$ is a slowly varying function of bounded variation in $(0,\lambda_0)$ with $L_{f,1}(\lambda) \to c \neq 0$ as $\lambda \to \lambda_0^-$. Then...
        \[
        \gamma_X(h) =
        \]
    \end{enumerate}
\end{proposition}

Let's start with the second claim.
\[
\int_0^{\lambda_0} \cos(h \lambda ) f_X(\lambda) d\lambda \sim  
c \int_0^{\lambda_0} \cos(h \lambda )  d\lambda = c \sin(h\lambda_0) h^{-1}.
\]
On the other hand, from previous calculations.
\[
\int_{\lambda_0}^\pi \cos(h \lambda ) f_X(\lambda) d\lambda \sim  
\Gamma(1-2d) L_{f,2}(h) (\cos(\pi d) - \sin(\pi d)) h^{2d-1}.
\]

With regard to the third claim
\begin{equation}
\begin{split}
    &\int_0^{\lambda_0} \cos(h \lambda ) f_X(\lambda) d\lambda \sim \int_0^{\lambda_0} \cos(h \lambda ) |\log((\lambda_0 - \lambda)^{-1})| d\lambda \\
    &= \cos(h \lambda_0) \int_0^{\lambda_0} \cos(h \om)  |\log \left( \frac{1}{\om} \right)|   d\om + \sin(h \lambda_0) \int_0^{\lambda_0} \sin(h \om)  |\log \left( \frac{1}{\om} \right)|   d\om \\
    &= - \cos(h \lambda_0) \int_0^{\lambda_0} \cos(h \om)  \log \left( \om \right)   d\om - \sin(h \lambda_0) \int_0^{\lambda_0} \sin(h \om)  \log \left( \om \right)   d\om \\
    % &\ \cos(h\lambda_0) \log(h) h^{-1} + \sin(h\lambda_0) h^{-1} = O\left(\frac{log(h)}{h}\right)
\end{split}
\end{equation}
Formular 4.381(1) and (2) of \cite{Graryz15},
\[
\int_0^1 \log (x) \sin (ax) dx = - \frac{1}{\alpha} \left[ C + log(\alpha) - ci(\alpha) \right], \quad \int_0^1 \log (x) \cos (ax) dx = - \frac{1}{\alpha} \left[  si(\alpha)  + \frac{\pi}{2} \right]
\]
where
\[
ci(\alpha) = - \int_\alpha^\infty \frac{cos(x)}{x} dx = C + \log(\alpha) + \int_0^\alpha \frac{\cos(t)-1}{t} dt
\]
and
\[
si(\alpha) = - \int_\alpha^\infty \frac{sin(x)}{x} dx  = 
 -\frac{\pi}{2} + \int_0^\alpha \frac{sin(t)}{t} dt 
\]
(last two formulars are 8.230 of \cite{Graryz15}). This says that, since $\lim_{a \to \infty} si(a) = \frac{\pi}{2}$
\[
- \cos(h \lambda_0) \int_0^{\lambda_0} \cos(h \om)  \log \left( \om \right)   d\om \sim \cos(h \lambda_0) \frac{1}{h}, \quad - \sin(h \lambda_0) \int_0^{\lambda_0} \sin(h \om)  \log \left( \om \right)   d\om \sim \sin(h \lambda_0) \frac{1}{h}.
\]


\PZ{
Under somewhat strict conditions on $L$ we have that as $\theta \to 0^+$,
\[
\sum_{n=1}^\infty L(n) \frac{\sin(n \theta)}{n^{\alpha}} \sim \frac{L(1/\theta)}{\theta^{1-\alpha}} \frac{\frac{1}{2}\pi}{\Gamma(\alpha)\sin(\frac{1}{2}\pi \alpha)}
\]
(see \cite{bingham_goldie_teugels_1987}, below equation (6.1) and also on the section for Abel summability for conditions on $L$). Allegedly this holds for $-1 < \alpha \le 0$ as well (under the stricter conditions), but this display doesn't make sense for the desired value $\alpha = 0$.
}



\begin{remark}
    Lemma 1 of Chapter 2 in \cite{phdArt98} provided a heuristic argument for 
\end{remark}
